# Supplementary material for: Human Detection and Segmentation via Multi-view Consensus
Source: arXiv:2012.05119 source file (2021-08-18)
Supplement: Supplementary file 1 [file appendix.tex]

\externaldocument{method.tex}
In this document, we present the details of our differentiable multi-view consistency formulation, architecture design, and training strategies. Furthermore, we show additional qualitative results on the $\textbf{Ski-PTZ}$, $\textbf{H36M}$ and \handheld{} datasets. We provide a video which can be accessed on \url{https://youtu.be/bg3AYjTa1NY} to explain the multi-view consistency setup and demonstrate the $\textbf{Ski-PTZ}$ and \handheld{} video results including the intermediate outputs of our method along with the detection and segmentation predictions on consecutive frames for all cameras and test subjects.
%Further qualitative results are shown in the supplemental video.
\section{Implementation Details}

\subsection{Multi-view Consistency}
\vspace{4mm}
\parag{Adjusting  Bounding Box Centers.}
The candidate object location proposed by the sampled grid cell in camera $c$ is defined as $\vb_c = [\delta x, \delta y, s_x, s_y]$ where $\delta x, \delta y \in [0, 1]$ are the offsets from the grid center and $s_x, s_y \in [0,1]$ are the width and height of the bounding box respectively. The center location of the proposal in pixel coordinates can be written as
\begin{equation}
\begin{aligned}
{u}_{c} &= W * \delta x + g_{x} \;,\\
{v}_{c} &= H * \delta y + g_{y}  \;,
\label{eq:bbox center}
\end{aligned}
\end{equation}
where ${u}_{c} \in [0, W]$, ${v}_{c} \in [0, H]$ and $g_{x} \in [0, W]$, $g_{y} \in [0, H]$ denote the grid center in pixel coordinates. To reach a multi-view consensus on the center of a 3D bounding box, namely $\textbf{\=u} \in {\mathbb{R}}^{3 \times 1}$, we take into account the lines emerging from camera positions $\textbf{o}_{c} \in {\mathbb{R}}^{3 \times 1}$ for each camera. The line of sight for the proposal center is calculated as
\begin{equation}
\vl_c =  \mM_c^{-1} \left[ \begin{array}{c} u_c \\ v_c \\ 1\end{array} \right] \;,
\label{eq:3dcenter}
\end{equation}
where $\vl_c$  represents all the points corresponding to the center of the sampled box in world coordinates relative to the camera center and $\mM_c$ is the $3 \times 3$ matrix formed by the first 3 columns of the projection matrix $\mP_c$. Note that we use bold symbols ($\vl_c$) for vectors in 3D world space and normal letters ($u$ and $v$) for coordinates in the 2D image plane. The unit direction vector for each of these lines is
\begin{equation}
\begin{aligned}
\textbf{n}_c &=  \frac{\vl_c}{\norm{\vl_c}} \;,
\label{eq:unit_direction}
\end{aligned}
\end{equation}
where $\textbf{n}_c \in  {\mathbb{R}}^{3 \times 1}$. To find the nearest point $\textbf{\=u}$ to a set of lines, we calculate the point with minimum distance to them. Given that each line is defined by its origin $\textbf{o}_{c}$ and the unit direction vector $\textbf{n}_c$, the squared perpendicular distance from the point $\textbf{\=u}$ to one of these lines is given by

\begin{equation}
\begin{aligned}
\textbf{d}_c &=  (\textbf{o}_{c}  - \textbf{\=u})^{T} (\bf I - \textbf{n}_c(\textbf{n}_c)^T)  (\textbf{o}_{c}  - \textbf{\=u}) \;,
\label{eq:distance}
\end{aligned}
\end{equation}
where the matrix $ (\bf I - \textbf{n}_c(\textbf{n}_c)^T) $ serves as the projector of the line vectors into the space orthogonal to $\textbf{n}_c$. By minimizing the sum of squared distances, we can obtain the nearest point in the least squares sense for $C$ cameras. The objective we want to minimize is
\begin{equation}
\begin{aligned}
\sum_{c=1}^{C} \textbf{d}_c &=  \sum_{c=1}^{C} (\textbf{o}_{c}  - \textbf{\=u})^{T} (\bf I - \textbf{n}_c(\textbf{n}_c)^T)  (\textbf{o}_{c}  - \textbf{\=u}) \;.
\label{eq:distance_sum}
\end{aligned}
\end{equation}
The derivative with respect to $\textbf{\=u}$ gives
\begin{equation}
\begin{aligned}
\sum_{c=1}^{C} -2 (\bf I - \textbf{n}_c(\textbf{n}_c)^T)   (\textbf{o}_{c}  - \textbf{\=u})  = 0 \;,
\label{eq:distance_sum_derivative}
\end{aligned}
\end{equation}
where $\bf I$ is the $3 \times 3$ identity matrix. Re-arranging this, we obtain a system of linear equations
\begin{equation}
\begin{aligned}
\bf A \textbf{\=u} &= \bf m \;,\\
\bf A &= \sum_{c=1}^{C} (\bf I - \textbf{n}_c(\textbf{n}_c)^T) \;, \\
\bf m &= \sum_{c=1}^{C} (\bf I - \textbf{n}_c(\textbf{n}_c)^T) \textbf{o}_{c} \;,
\label{eq:lstsq}
\end{aligned}
\end{equation}
with $\bf A \in {\mathbb{R}}^{3 \times 3}$ and $\bf m \in  {\mathbb{R}}^{3 \times 1}$.  The optimum is achieved at the least squares solution. Therefore, $\textbf{\=u} = lstsq(\bf A, \bf m)$ and we use a differentiable implementation of $\textit{lstsq}$ function to solve it. 

The new center computed through multi-view consistency is projected onto each view to update the value of the 2D bounding box centers. Thus, 
\begin{equation}
\begin{aligned}
\begin{bmatrix}
{\bar{u}}_c \\
{\bar{v}}_c \\
1
\end{bmatrix}
= \textbf{M}_{c} \textbf{\=u} \;,
\end{aligned}
\label{eq:new_center_2D}
\end{equation}
where $ \textbf{\=u}$ represents the coordinates of the new center in 3D and $ \{{\bar{u}}_c, {\bar{v}}_c\}$ are the updated 2D bounding box centers in each view.\\

\parag{Adjusting Bounding Box Heights.} 
Similarly, the top and bottom points of the 2D bounding boxes can be subject to the multi-view consistency. The top and bottom locations, $\{{u}_{t,c}  , {v}_{t,c}\}$ and $\{{u}_{b,c}, {v}_{b,c}\}$ respectively, of the bounding box in camera view $c$ are computed as
\begin{equation}
\begin{aligned}
{u}_{t,c} &= W * \delta x + g_{x} \;,\\
{v}_{t,c} &= H * \delta y  + g_{y} - (H * s_x)/2 \;,\\
{u}_{b,c} &= W * \delta x  + g_{x} \;,\\
{v}_{b,c} &= H * \delta y + g_{y} + (H * s_x)/2 \;.
\label{eq:bbox top_bottom}
\end{aligned}
\end{equation}
To find the consensus top and bottom locations in 3D, we apply the least squares solution explained in the previous section separately to the top and bottom points. For the top point, we consider the set of lines originating from camera positions $\textbf{o}_{c} \in {\mathbb{R}}^{3 \times 1}$ for each camera. The line of sight for the top and bottom points of the bounding box in camera view $c$ are given as
\begin{equation}
\begin{aligned}
\vl_{t,c} =  \mM_c^{-1} \left[ \begin{array}{c} u_{t,c} \\ v_{t,c} \\ 1\end{array} \right] \;,\\
\vl_{b,c}=  \mM_c^{-1} \left[ \begin{array}{c} u_{b,c} \\ v_{b,c} \\ 1\end{array} \right] \;.
\label{eq:3dtop_bottom}
\end{aligned}
\end{equation}
To find the nearest point $\textbf{\={u}}_{t}$ to these lines, we apply Eq.~\ref{eq:unit_direction},~\ref{eq:distance},~\ref{eq:distance_sum},~\ref{eq:distance_sum_derivative} and~\ref{eq:lstsq}. Finally, we obtain the updated pixel location for the top point of the bounding box as follows
\begin{equation}
\begin{aligned}
\begin{bmatrix}
{\bar{u}}_{t,c} \\
{\bar{v}}_{t,c} \\
1
\end{bmatrix}
= \textbf{M}_{c} \textbf{\=u}_{t} \;.
\end{aligned}
\label{eq:new_top_2D}
\end{equation}
We update the 2D bottom location using the same multi-view least-squares strategy.
\subsection{Architectures}
Our main network $\cF$ consists of a detection and a synthesis network that reconstruct the input scene against the background image generated by the inpainting network.
\paragraph{Detection network.}  We predict one candidate bounding box relative to each 2D grid cell in a regular $8 \times 8$ grid using a fully-convolutional architecture similar to YOLO~\cite{Redmon16}. We use a ResNet-18 backbone \cite{He16a} without pre-training, that reduces the input dimensionality by a factor 16, forming a low resolution grid of features, e.g., to spatial resolution $8\times8$ from $128\times128$. The feature size is set to 5; two for bounding box location offset $\delta x, \delta y \in [0, 1]$ , two for scale $s_x, s_y \in [0,1]$, and one for the probability $p$. Each feature output represents the bounding box parameters predicted by one grid cell, and the offset is relative to the cell center $\{g_{x}, g_{y}\}$. The output $p$ is forced to be positive and form a proper distribution, with $\sum^{N}_{i=1} p_i = 1$ where $N = 64$, by a soft-max activation unit. To prevent this network from constantly predicting bounding boxes at the borders of the image, we zero out the outer cell probabilities.

\vspace{-3mm}
\paragraph{Synthesis network.}
This network takes as input the cropped image region corresponding to the sampled bounding box and has the form of a bottle-neck auto-encoder, based on the publicly available implementation of~\cite{Rhodin18b}.
The encoding part is a 50-layer residual network, and the weights are initialized with ones trained on ImageNet classification. The hidden layer is 856 dimensional, split into a 600 dimensional space and a 256 dimensional space that is replicated spatially to a $512\times8\times8$ feature map to encode spatially invariant features.
The decoding is done with the second half of a U-Net architecture with 64, 128, 256, 512 feature channels in each stage.
The final network layer outputs four feature maps, three to predict the color image $\hat{\mI} \in \R^{128 \times 128 \times 3}$ and one for the segmentation mask $\mS \in \R^{128 \times 128}$.

%\paragraph{Discussion.}
%We use a YOLO detection architecture combined with spatial transformers and the synthesis network $\cS$. To improve inference speed, one could merge $\cD$ and $\cS$ to share the same base network through RoI pooling as in MaskRCNN. Nevertheless, the MC training approach is necessary, because the inpainting network $\cI$, discussed below, cannot share the same features for multiple bounding box locations as the blacked-out input region varies for each $\vb_c$.

\vspace{-3mm}
\paragraph{Inpainting network.}

The inpainting network is trained separately for each dataset, from scratch and on the training split, without requiring any annotation. It is a 6 layer U-Net model with 8, 16, 32, 64, 128, 256 feature channels in each stage. It is trained independently from the rest of the pipeline by feeding images with randomly occluded regions of varying sizes. To compare the reconstructed image $\mI'$ to the original one $\mI$, we use the $\loss_2$ pixel reconstruction and perceptual losses
\begin{align}
\loss_{reconst} &= ||\mI - \mI'||^2 \;,\\
\loss_{perc} &= ||\phi(\mI) - \phi(\mI')||^2 \;,
\end{align}
where $\phi(.)$ indicates the low level features obtained by passing its input to a pre-trained ResNet18 network. The pixel reconstruction and perceptual losses are weighted 1:2.

We integrate the inpainting network to our full pipeline and use it in an off-the-shelf manner. The input to the inpainter is an image where the selected bounding box region is hidden and the output is the entire image with the initially hidden patch being reconstructed. In our full pipeline, the weights of the inpainting network are frozen and to remove the image evidence corresponding to the foreground person, the hidden patch in the input image to the inpainting network is selected to be the bounding box region expanded by $15\%$ in both dimensions.

\subsection{Training Details}
\paragraph{Overall training.}

We train our model with $\loss_2$ pixel reconstruction and perceptual losses on the reconstructed image $\cF(\mI_c)$ and the $\loss_2$ pixel reconstruction loss on the inpainted background image $\bar{\mI}_c$ in view $c$ . We rely on the same prior terms as in~\cite{Katircioglu20} to regularize the predicted segmentation masks and probability values for the voxels. We use an $\loss_{seg}$ prior, which encourages the mean value of a segmentation mask to be larger than a threshold lambda but small in general,
\begin{equation}
\loss_{seg} = \left|\left(\frac{1}{WH}\sum^{W}_{x}\sum^{H}_{y}{\cT^{-1}(\mS)}_{xy} \right) - \lambda\right|+ \lambda \;,
\label{eq:v_prior}
\end{equation}
where $\lambda$ is set to 0.005 and the notation is the same as in the main paper. It encourages a non-zero segmentation mask at the beginning of the training, when the decoder still produces non-perfect foreground, which improves and stabilizes convergence. The voxel probabilities $q_j$ are regularized with
\begin{equation}
\loss_{q} = \sum_{j}^{V}|q_j|
\label{eq:q_prior}
\end{equation}
that favors only few voxels to have non-zero values. The total training loss we minimize can be written as
\begin{equation}
\begin{aligned}
\loss_{total} = & -  \alpha \sum_{c=1}^{C} r_j \frac{\|\bar{\mI}_c - \mI_c \|^2}{area(\vb^c_{i^{c}(j)})}  \\ 
					  & + \beta \sum_{c=1}^{C} r_j \| \cF(\mI_c) - \mI_c \|^2 \\ 
					  & + \gamma \sum_{c=1}^{C} r_j \| \phi(\cF(\mI_c)) - \phi(\mI_c) \|^2  \\ 
					  & + \eta \sum_{c=1}^{C}\loss_{seg}^{c} +  \zeta \loss_{q}
\label{eq:q_prior}
\end{aligned}
\end{equation}
where $\alpha=0.1, \beta=1, \gamma=2, \eta=0.25, \zeta=0.1$ and $\phi(.)$ indicates the low level features obtained by passing its input to a pre-trained ResNet18 network. The first three terms of $\loss_{total}$ correspond to $\objBG(\mI_1, \ldots, \mI_C)$, $\objFG (\mI_1, \ldots, \mI_C)$ and the perceptual version of $\objFG (\mI_1, \ldots, \mI_C)$ defined in Section {\color{red}3.1.4} of the main document.

As a baseline (\textit{Ours  w/ TC}), we report the results of using a $\loss_2$ loss term to minimize the distance between lines passing through the initial bounding box centers and camera optical centers in each view. 

All training stages are performed on a single NVIDIA TITAN X Pascal GPU with Adam and a learning rate of 1e-3. First, the inpainting network is optimized for 100k iterations and subsequently the complete network for an additional 50k iterations. The decoding part of the synthesis network uses a reduced learning rate of 1e-4, to prevent occasional diverging behavior. We use a batch size of 48 and an input image resolution of 640px$\times$360px for the \ski{} and \handheld{} and 500px$\times$500px for \human{}.
\vspace{-3mm}
\paragraph{Importance sampling.} Sampling from a discrete distribution is not differentiable with respect to its
parameters. Therefore, we integrate importance sampling as in~\cite{Katircioglu20}. However, instead of sampling from a 2D grid of cells, we sample a voxel from a 3D grid of proposals. Importance sampling allows us to introduce an auxiliary distribution $k$ that is used as the importance sampling distribution while maintaining the differentiability and optimizing the voxel probability distribution $q$. The relationship between $k$ and $q$ can be expressed as 
\begin{equation}
k_j = q_j (1 - V \epsilon) + \epsilon 
\end{equation}
for a voxel $j$, where $(1 - V \epsilon)$ determines the probability of choosing a random voxel.
In the multi-view setting, the number of voxels that can be seen by all the cameras change from one frame to another. Therefore the importance sampling related hyper-parameters must be adjusted accordingly. As in~\cite{Katircioglu20}, we take $(1 - V \epsilon) = 0.064$ and to satisfy this equality, we use an adaptive $\epsilon \approx 0.0002$, which makes the method numerically stable while the probability of choosing a random bounding box stays low, i.e., $6.4 \%$ for on average $V = 300$ voxels that participate the multi-view consensus voting. In Section {\color{red}3.1.4} of the main document, $r_j$ is the ratio of the probability $q_j$ by its importance sampling probability $k_j$.

\vspace{-3mm}
\paragraph{Consistency.}
We demonstrate that the proposed training strategy is stable and produces consistent results when repeated using the same configuration. To this end, we train the best-performing model on the $\textbf{Ski-PTZ}$ and $\textbf{H36M}$ datasets three times from scratch and provide the mean and std of the scores on the test sequences. The J- and F- measures on the $\textbf{Ski-PTZ}$ dataset are consistent, respectively, $0.71 \pm 0.006$, $0.83 \pm 0.002$ and the mAP$_{0.5}$ score on $\textbf{H36M}$ dataset is $0.85 \pm 0.004$.

\comment{
\paragraph{Regression vs. classification.} In principle, the bounding box position could be regressed per view, without the proposal network and 3D voting. However, the application to unknown moving backgrounds in \cite{Katircioglu20} and  in our own solution requires optimizing the background objective of Eq.~\ref{eq:background objective} with respect to discrete proposals. With a pure regression network, the training drifts towards trivial solutions of overly large bounding boxes that maximize Eq.~\ref{eq:background objective} while violating the main objective Eq.~\ref{eq:expected objective}. 
}

\section{Qualitative Results}

We present additional qualitative results on \ski{}, \human{} and \handheld{} in Fig.~\ref{fig:supp_ski_qual}, Fig.~\ref{fig:supp_h36m_qual} and Fig.~\ref{fig:supp_handheld_qual} respectively. On \ski{}, our method reliably detects the skier even when there are other people in the scene and our segmentation predictions cover the entire body and skis more accurately than~\cite{Yang19c}, relying on multi-view consistency

\begin{figure*}[hbt!]
  \centering
  {

  \begin{tabular}{@{}cccccc@{}}

   \includegraphics[width=0.16\linewidth]{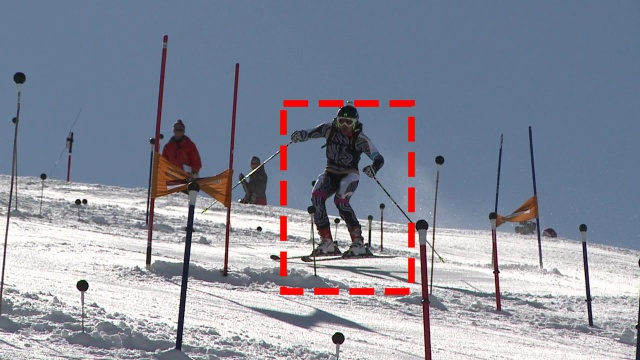} &\hspace{-4.0mm}
   \includegraphics[width=0.16\linewidth]{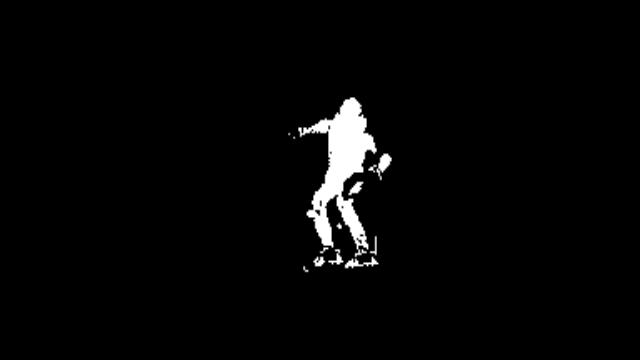} &\hspace{-4mm}
   \includegraphics[width=0.16\linewidth]{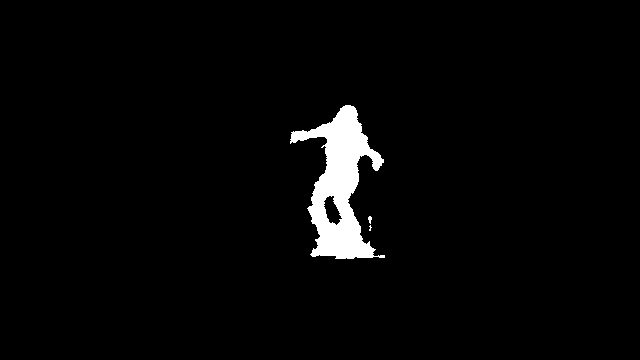} &\hspace{-4mm}
   \includegraphics[width=0.16\linewidth]{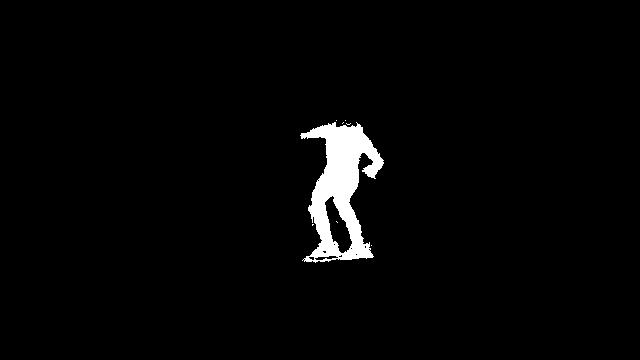} &\hspace{-4mm}
   \includegraphics[width=0.16\linewidth]{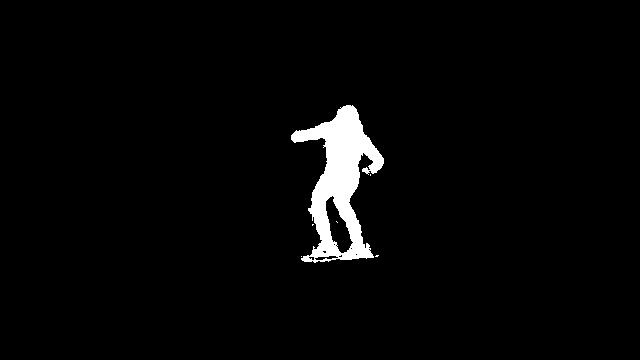} &\hspace{-4mm}
   \includegraphics[width=0.16\linewidth]{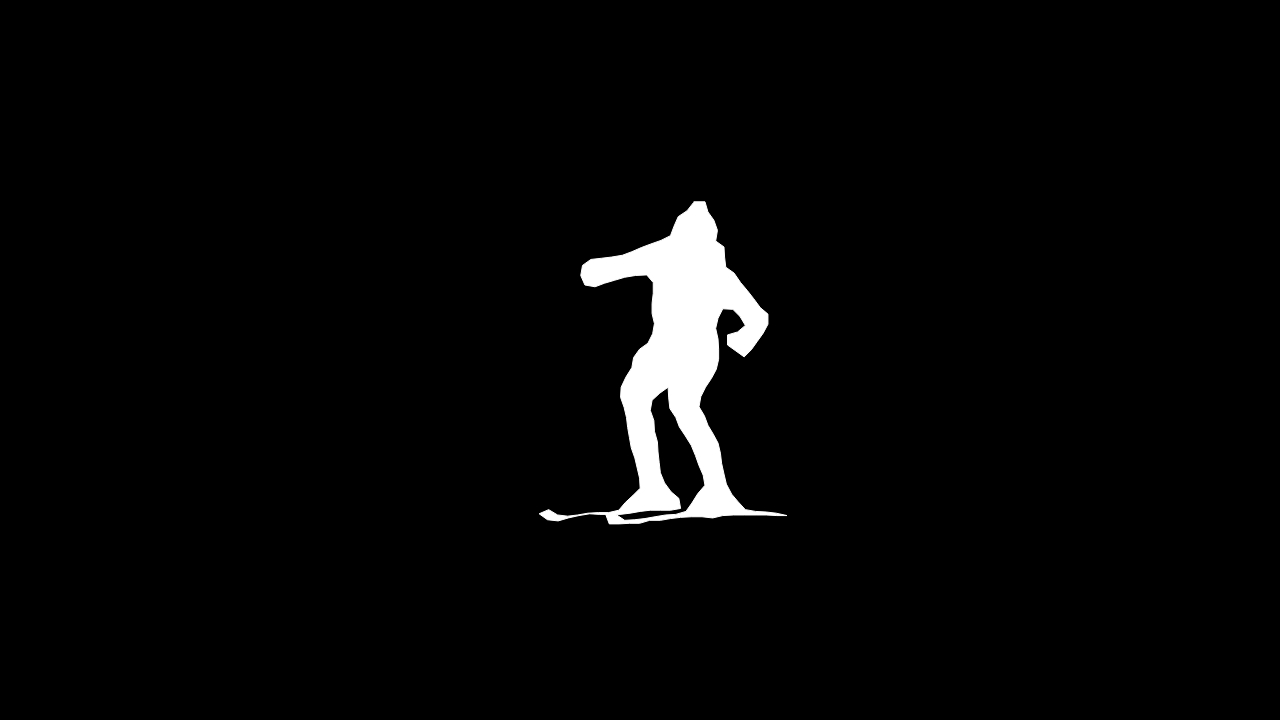} \\

    \includegraphics[width=0.16\linewidth]{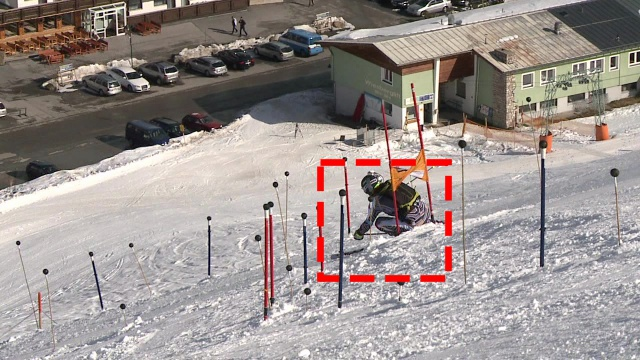} &\hspace{-4.0mm}
   \includegraphics[width=0.16\linewidth]{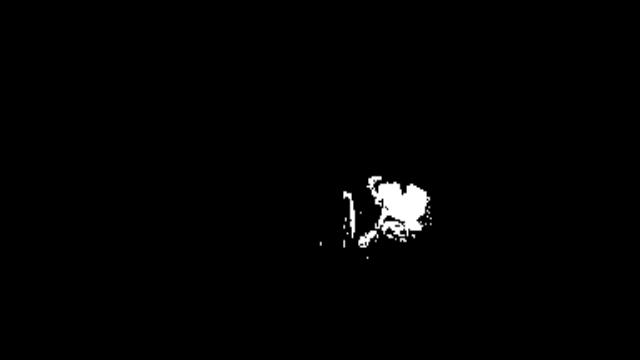} &\hspace{-4mm}
   \includegraphics[width=0.16\linewidth]{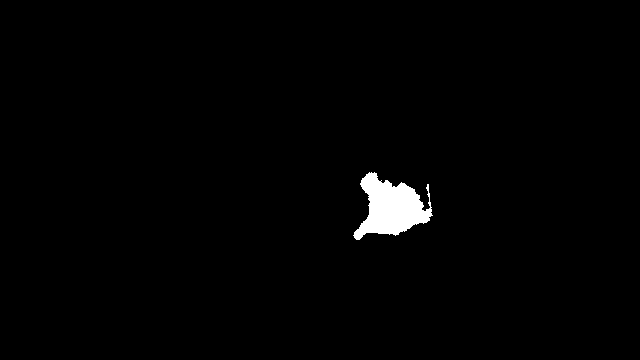} &\hspace{-4mm}
   \includegraphics[width=0.16\linewidth]{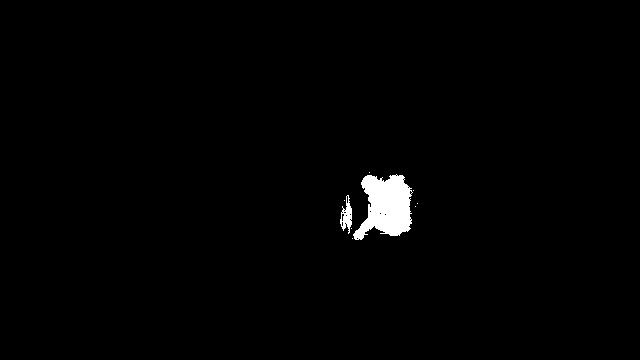} &\hspace{-4mm}
   \includegraphics[width=0.16\linewidth]{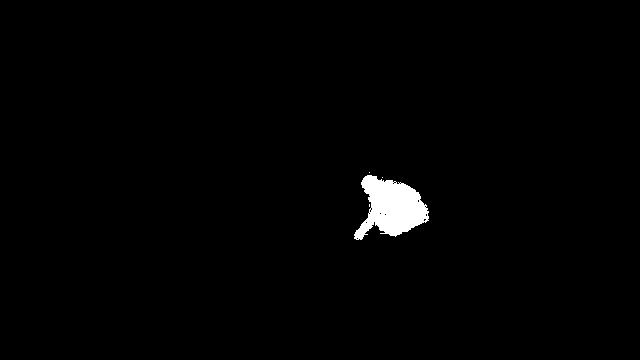} &\hspace{-4mm}
   \includegraphics[width=0.16\linewidth]{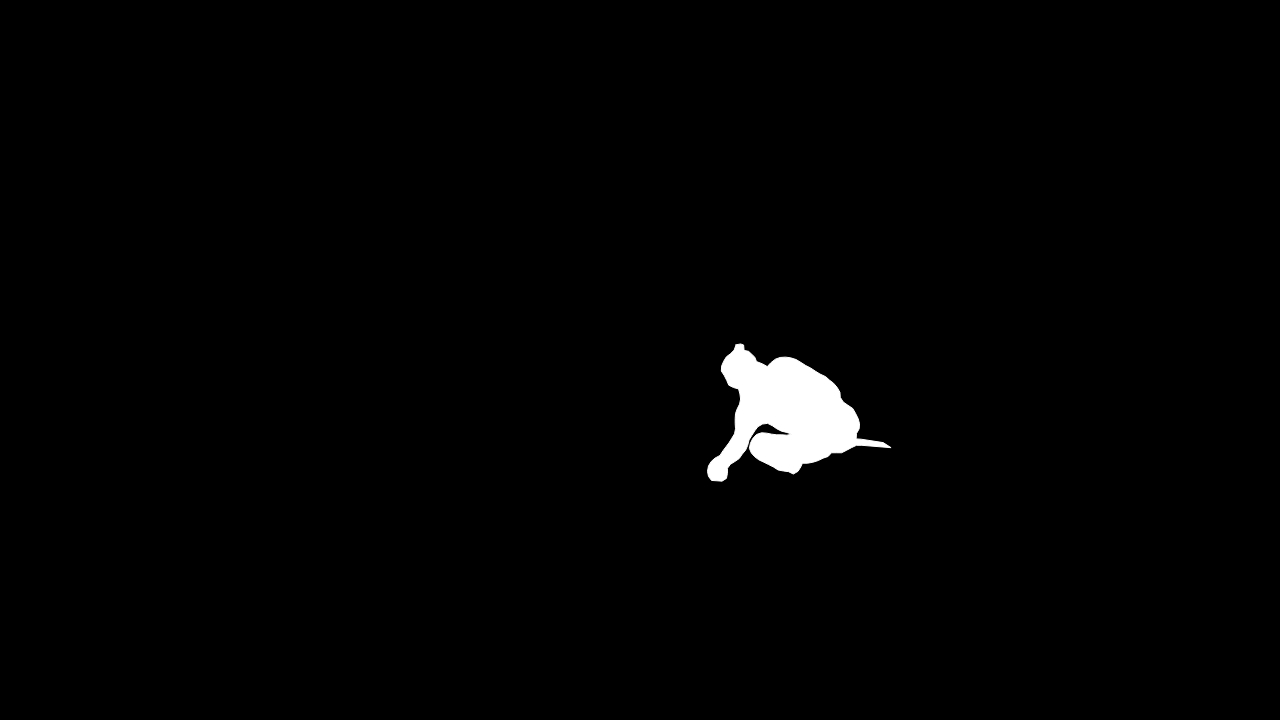} \\

   \includegraphics[width=0.16\linewidth]{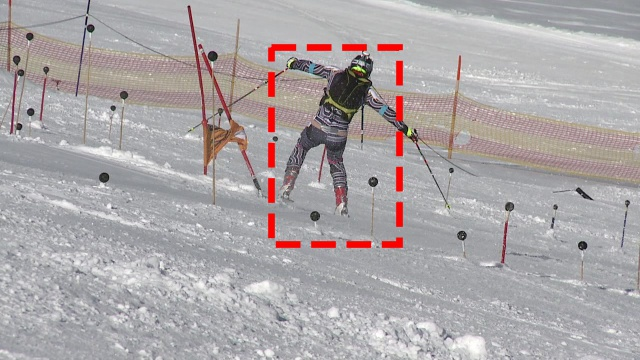} &\hspace{-4.0mm}
   \includegraphics[width=0.16\linewidth]{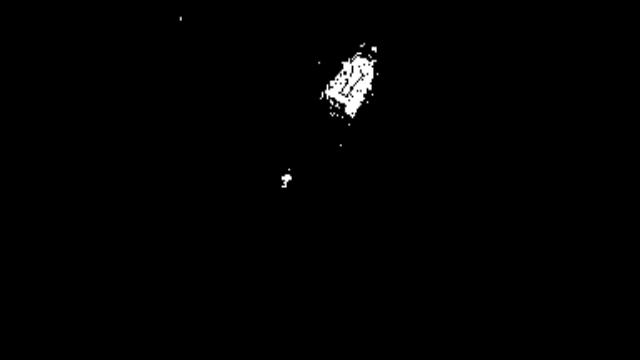} &\hspace{-4mm}
   \includegraphics[width=0.16\linewidth]{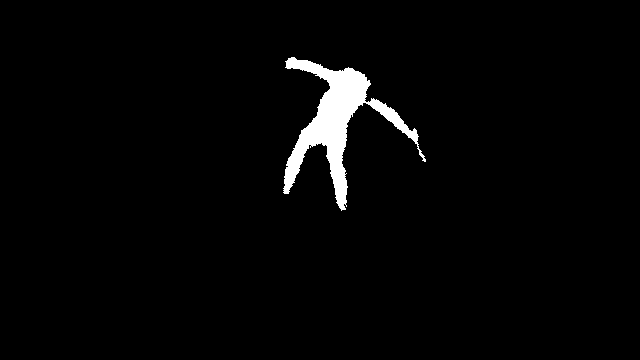} &\hspace{-4mm}
   \includegraphics[width=0.16\linewidth]{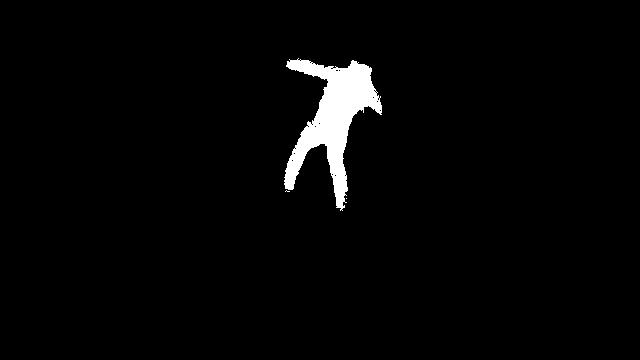} &\hspace{-4mm}
   \includegraphics[width=0.16\linewidth]{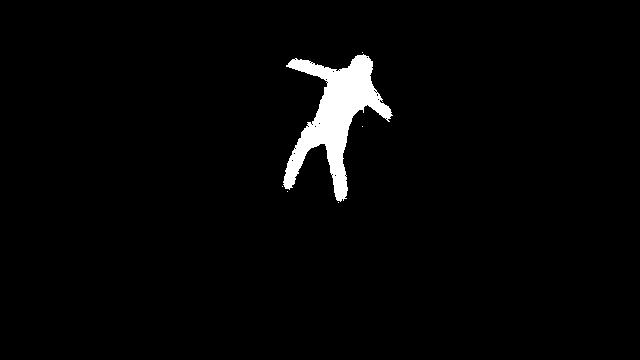} &\hspace{-4mm}
   \includegraphics[width=0.16\linewidth]{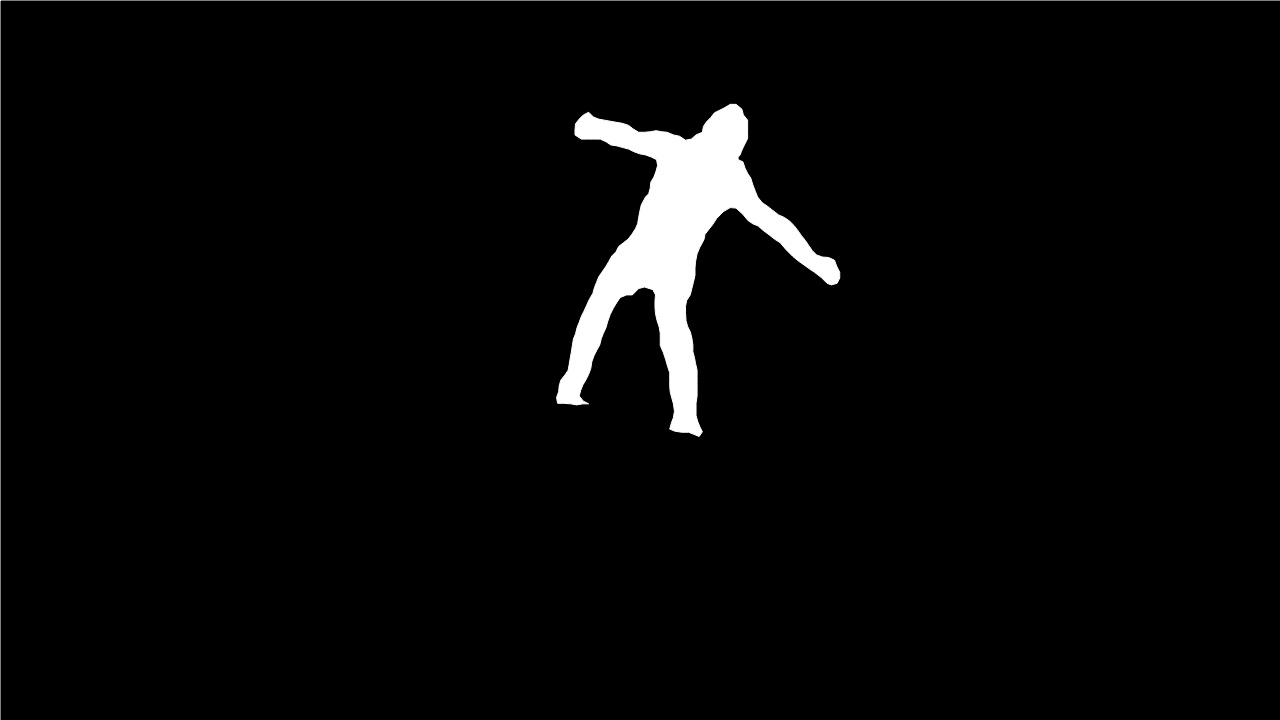} \\

    \includegraphics[width=0.16\linewidth]{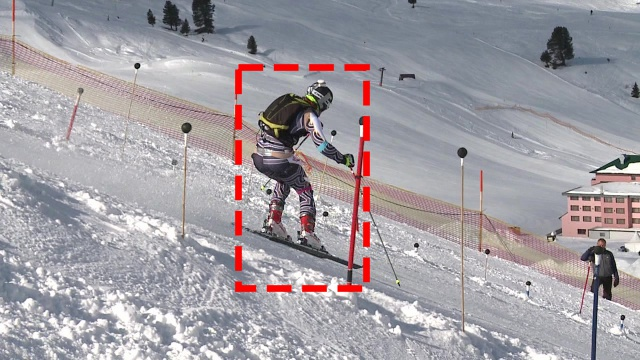} &\hspace{-4.0mm}
   \includegraphics[width=0.16\linewidth]{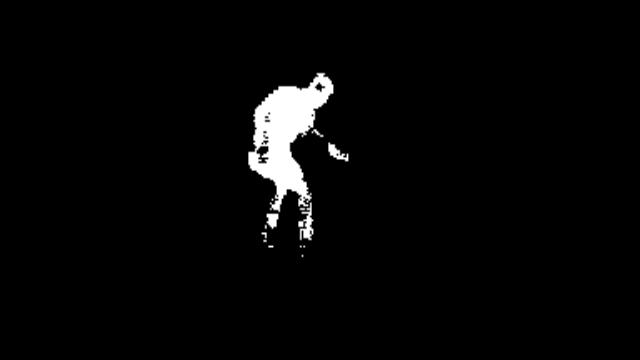} &\hspace{-4mm}
   \includegraphics[width=0.16\linewidth]{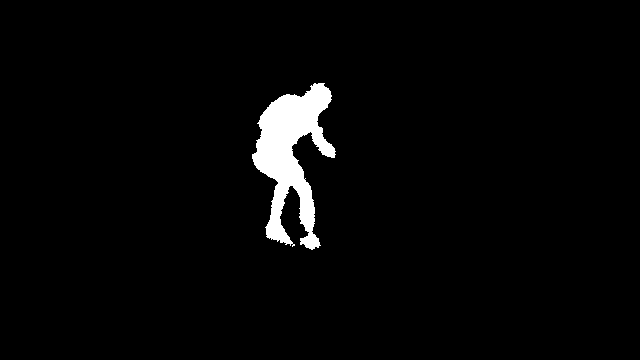} &\hspace{-4mm}
   \includegraphics[width=0.16\linewidth]{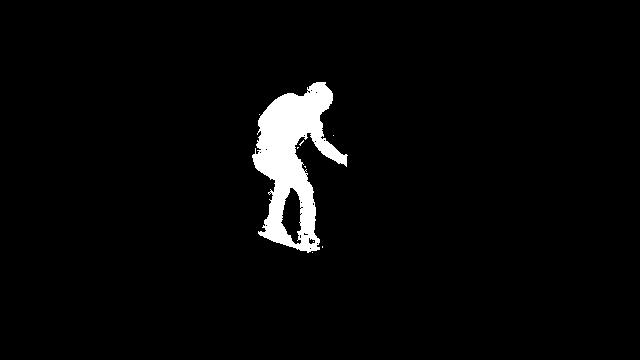} &\hspace{-4mm}
   \includegraphics[width=0.16\linewidth]{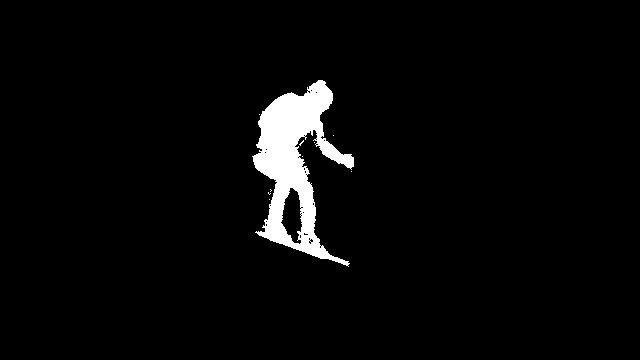} &\hspace{-4mm}
   \includegraphics[width=0.16\linewidth]{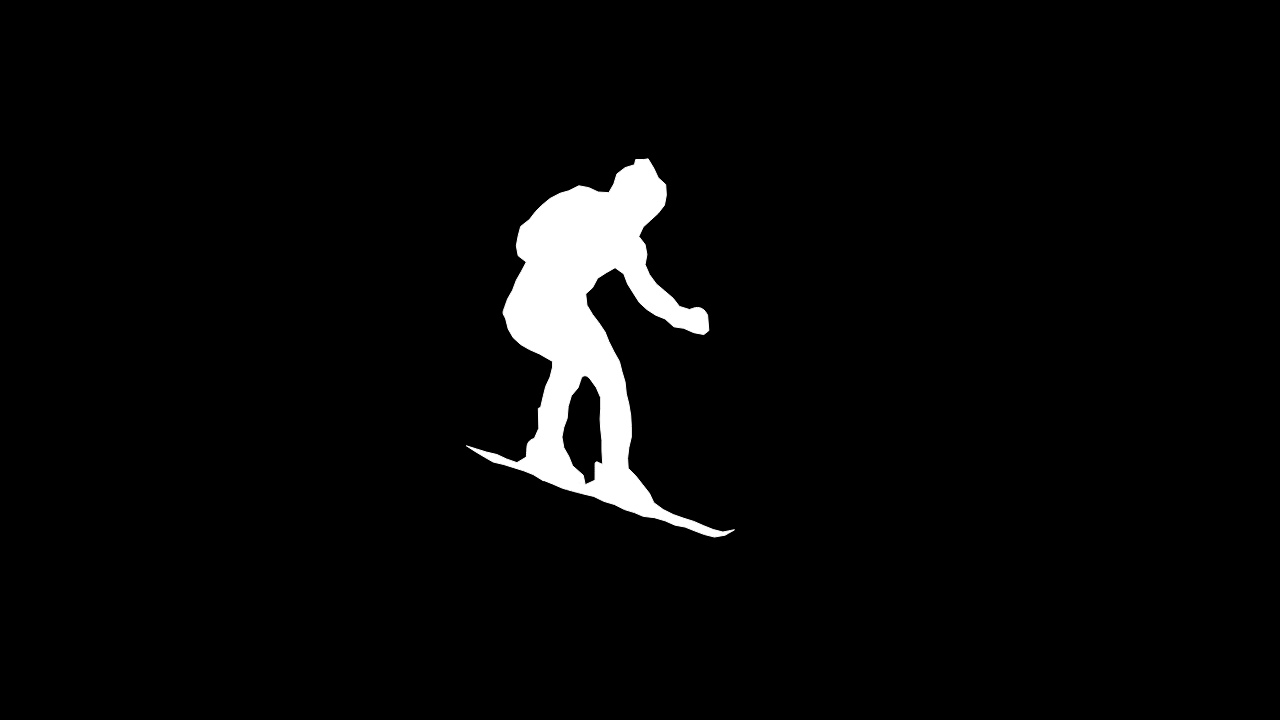} \\

   \includegraphics[width=0.16\linewidth]{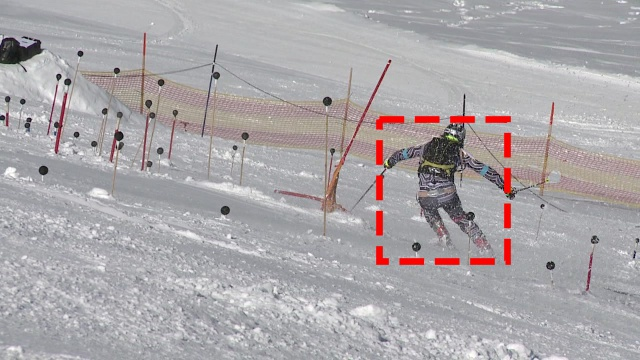} &\hspace{-4.0mm}
   \includegraphics[width=0.16\linewidth]{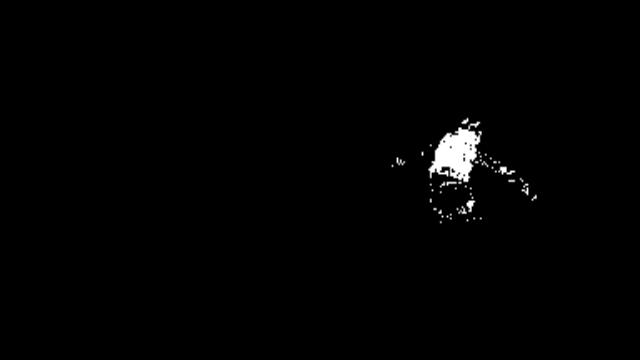} &\hspace{-4mm}
      \includegraphics[width=0.16\linewidth]{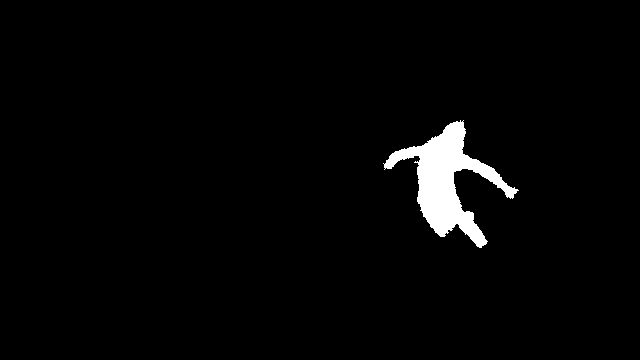} &\hspace{-4mm}
   \includegraphics[width=0.16\linewidth]{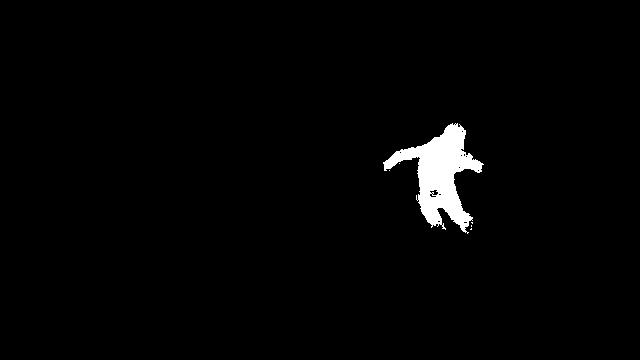} &\hspace{-4mm}
   \includegraphics[width=0.16\linewidth]{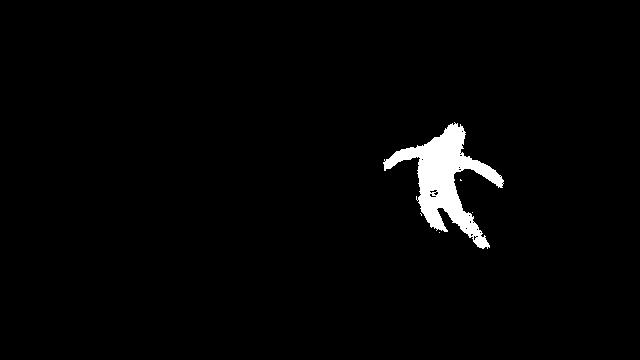} &\hspace{-4mm}
   \includegraphics[width=0.16\linewidth]{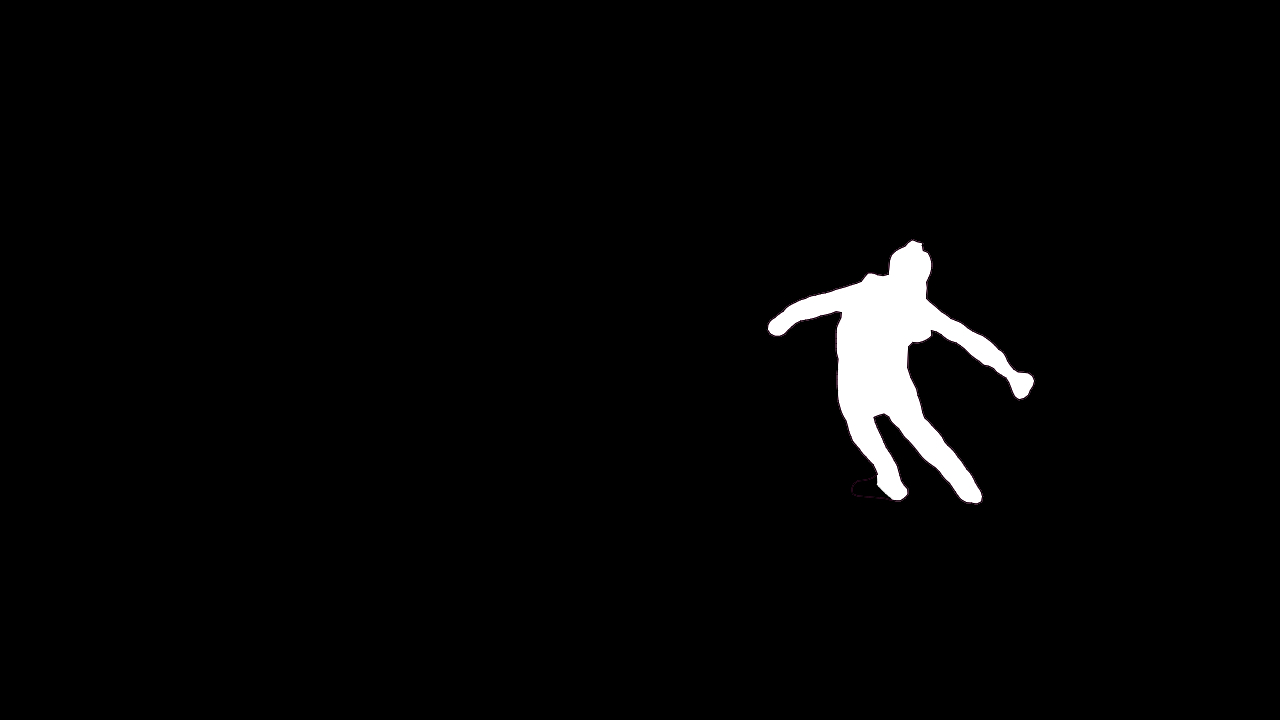} \\

  \includegraphics[width=0.16\linewidth]{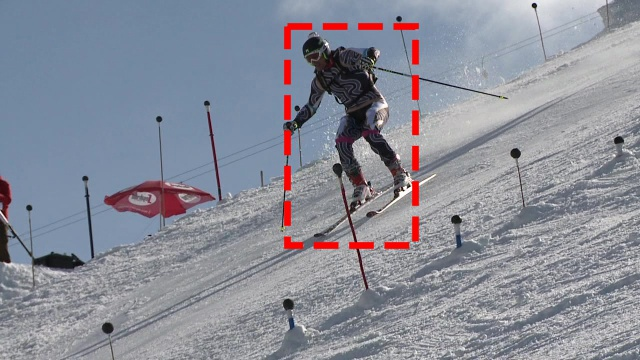} &\hspace{-4.0mm}
  \includegraphics[width=0.16\linewidth]{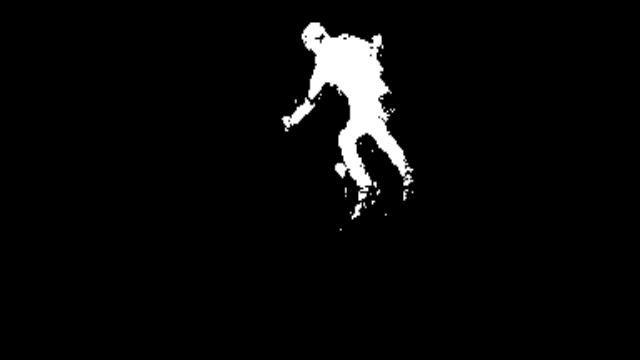}& \hspace{-4mm}
     \includegraphics[width=0.16\linewidth]{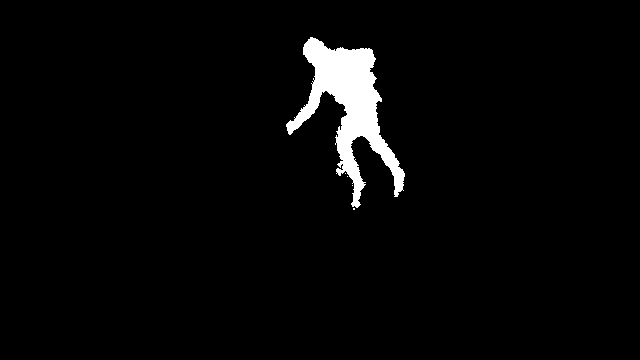}& \hspace{-4mm}
  \includegraphics[width=0.16\linewidth]{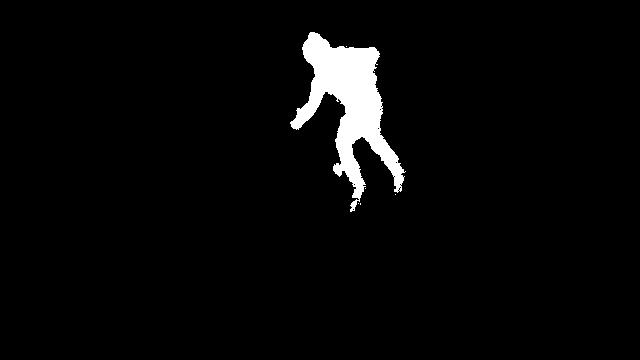}& \hspace{-4mm}
    \includegraphics[width=0.16\linewidth]{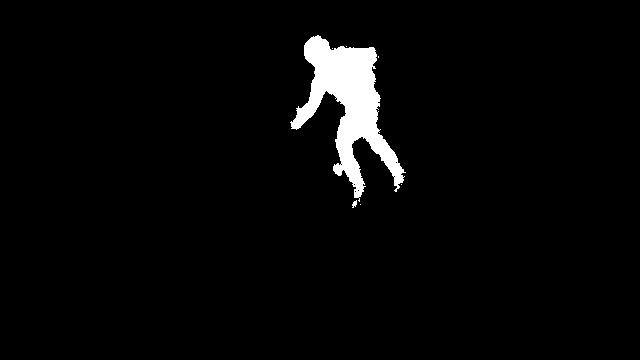}& \hspace{-4mm}
  \includegraphics[width=0.16\linewidth]{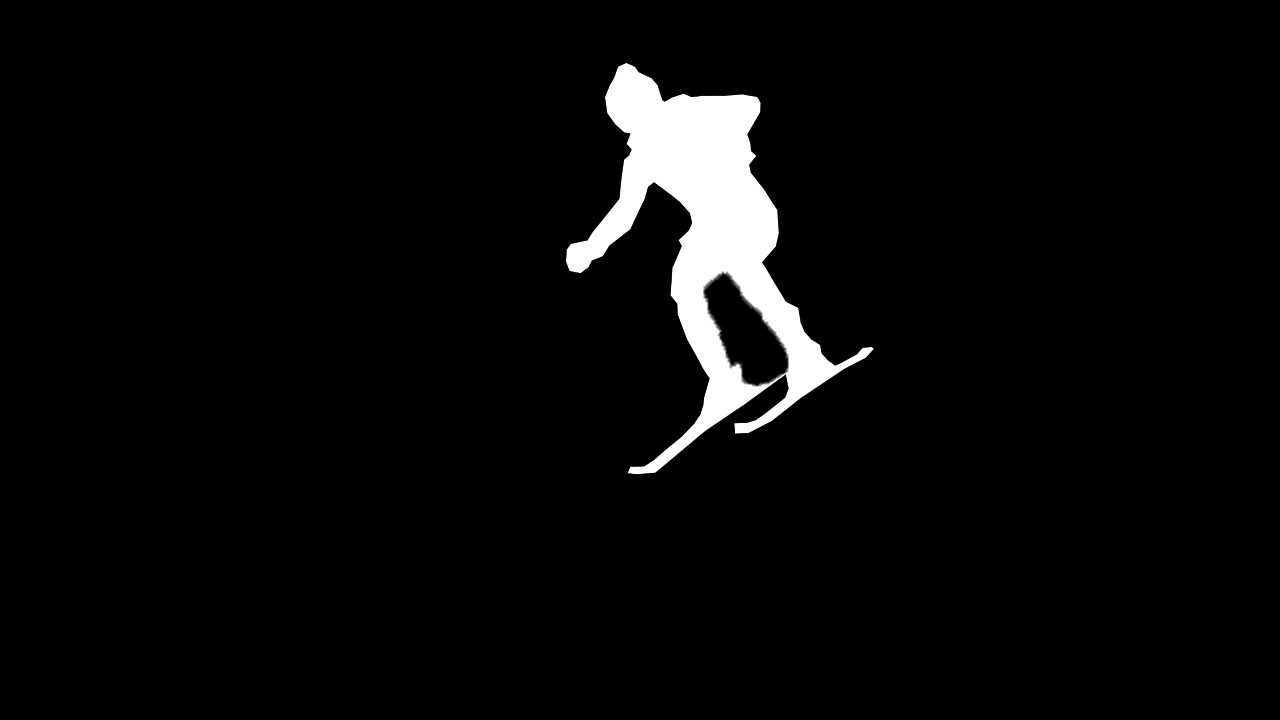}  \\
  
  \includegraphics[width=0.16\linewidth]{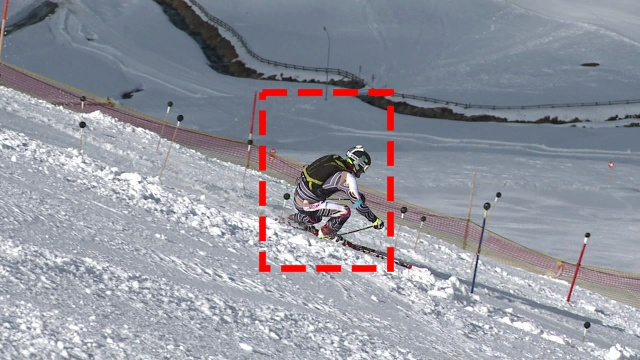} &\hspace{-4.0mm}
  \includegraphics[width=0.16\linewidth]{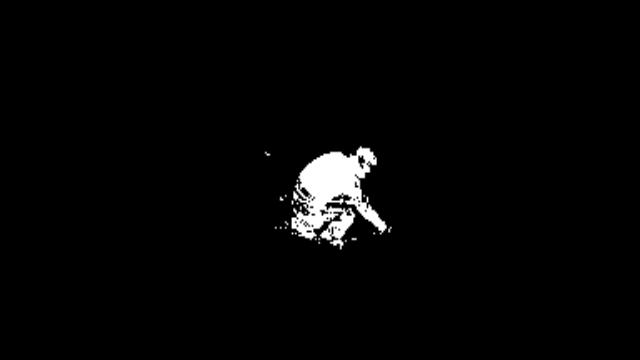}& \hspace{-4mm}
  \includegraphics[width=0.16\linewidth]{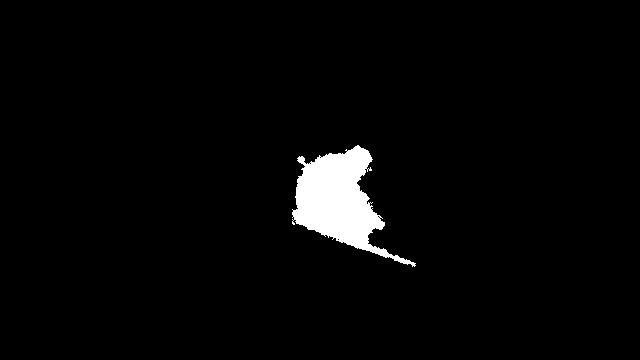}& \hspace{-4mm}
  \includegraphics[width=0.16\linewidth]{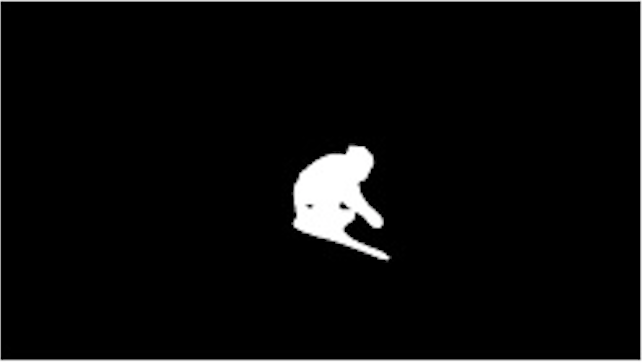}& \hspace{-4mm}
    \includegraphics[width=0.16\linewidth]{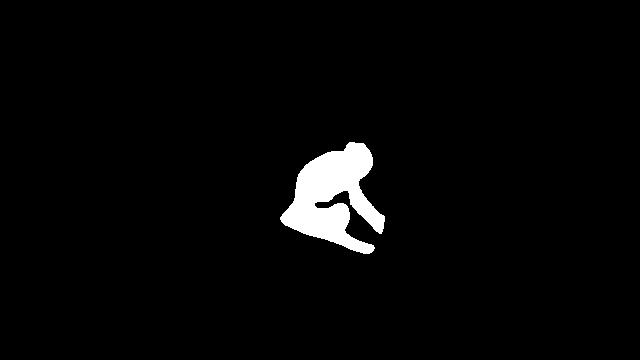}& \hspace{-4mm}
  \includegraphics[width=0.16\linewidth]{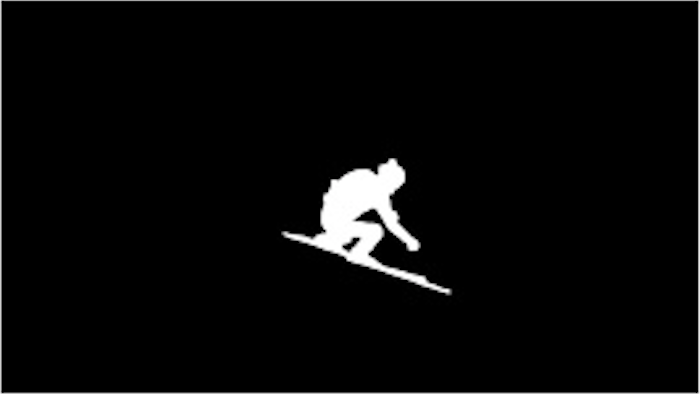}  \\

\includegraphics[width=0.16\linewidth]{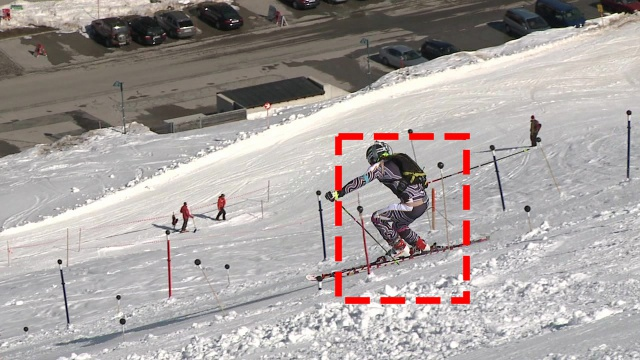} &\hspace{-4.0mm}
\includegraphics[width=0.16\linewidth]{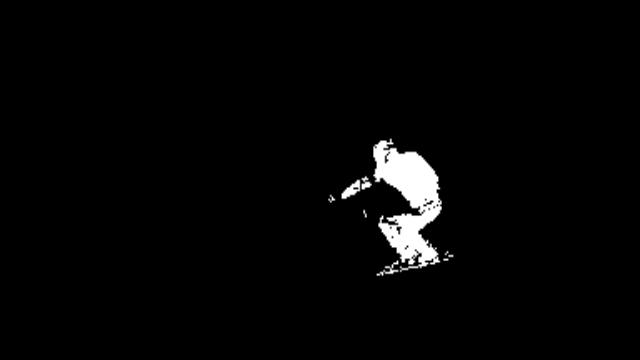} &\hspace{-4mm}
\includegraphics[width=0.16\linewidth]{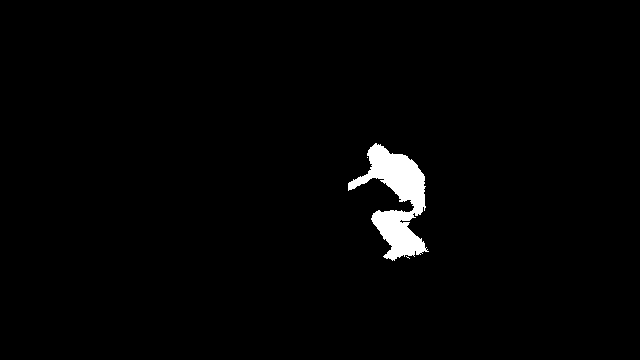} &\hspace{-4mm}
\includegraphics[width=0.16\linewidth]{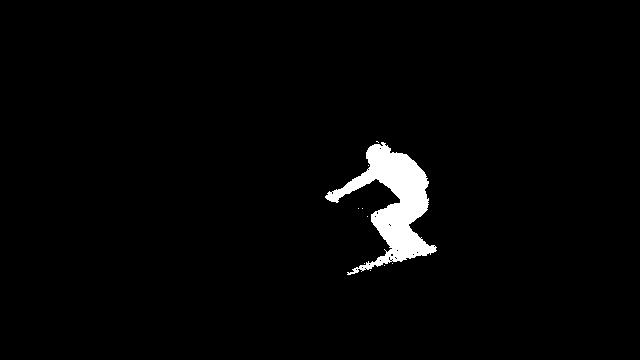} &\hspace{-4mm}
\includegraphics[width=0.16\linewidth]{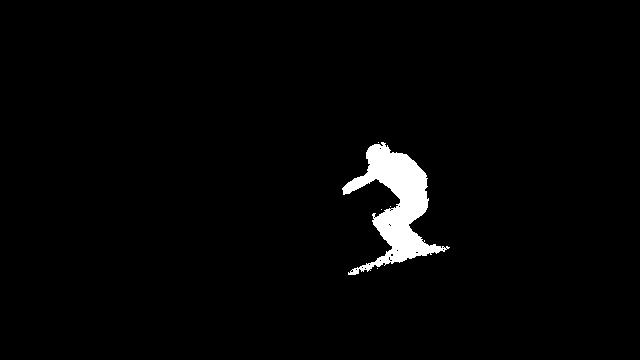} &\hspace{-4mm}
\includegraphics[width=0.16\linewidth]{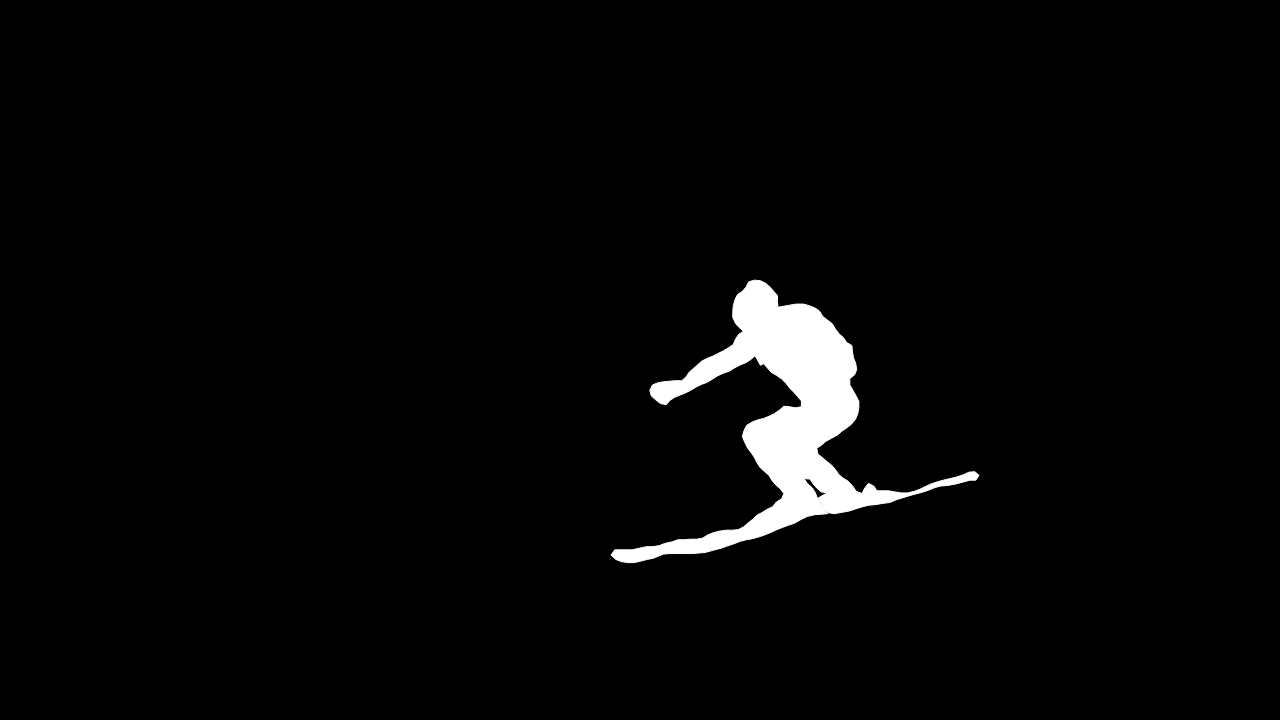} \\ 

\includegraphics[width=0.16\linewidth]{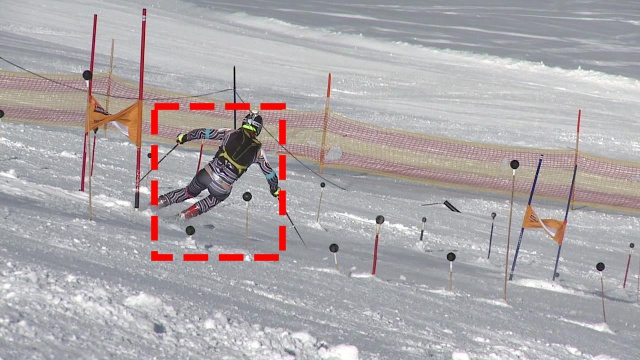} &\hspace{-4.0mm}
\includegraphics[width=0.16\linewidth]{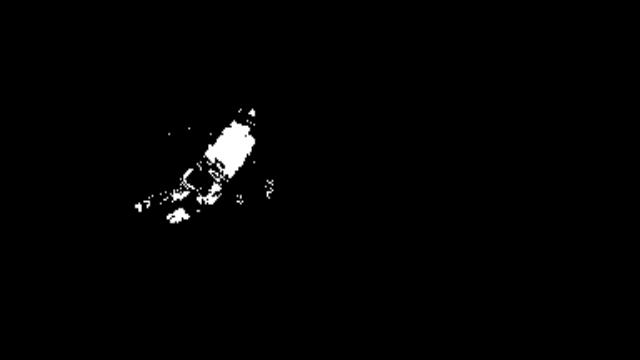} &\hspace{-4mm}
\includegraphics[width=0.16\linewidth]{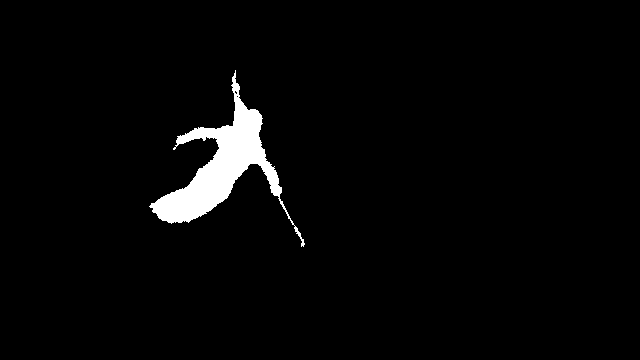} &\hspace{-4mm}
\includegraphics[width=0.16\linewidth]{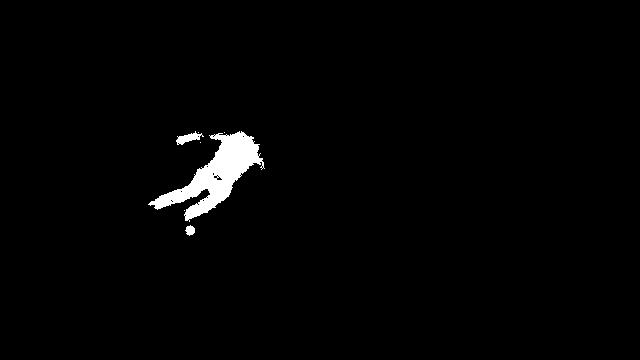} &\hspace{-4mm}
\includegraphics[width=0.16\linewidth]{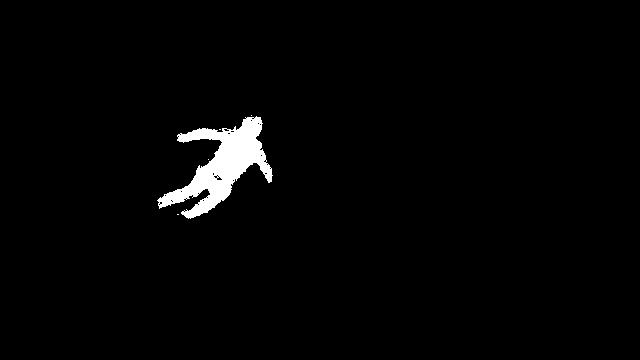} &\hspace{-4mm}
\includegraphics[width=0.16\linewidth]{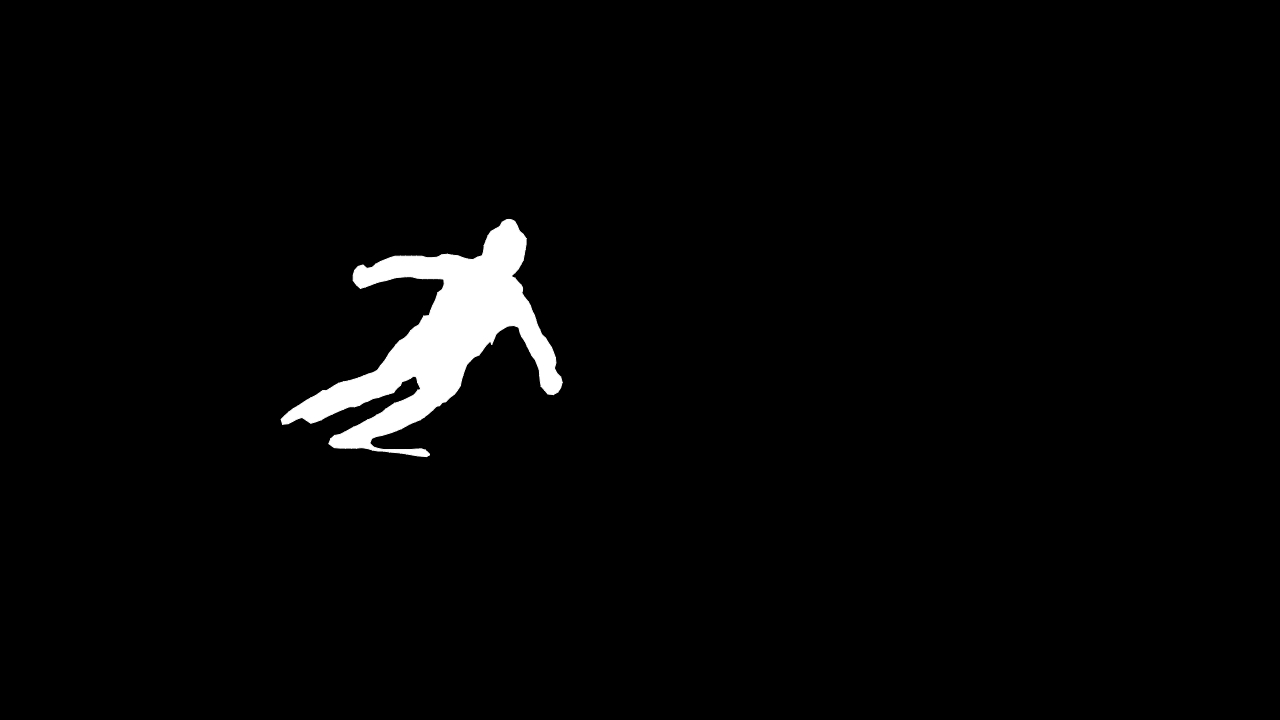} \\

\includegraphics[width=0.16\linewidth]{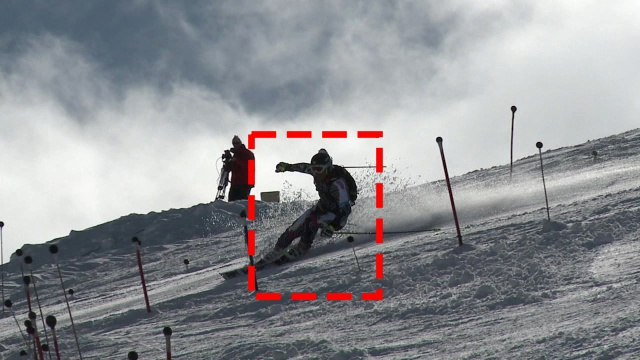} &\hspace{-4.0mm}
\includegraphics[width=0.16\linewidth]{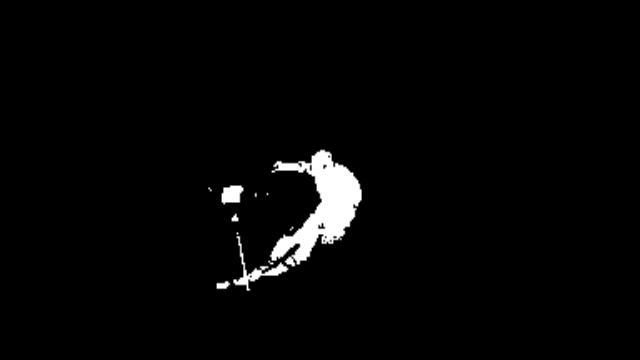} &\hspace{-4mm}
\includegraphics[width=0.16\linewidth]{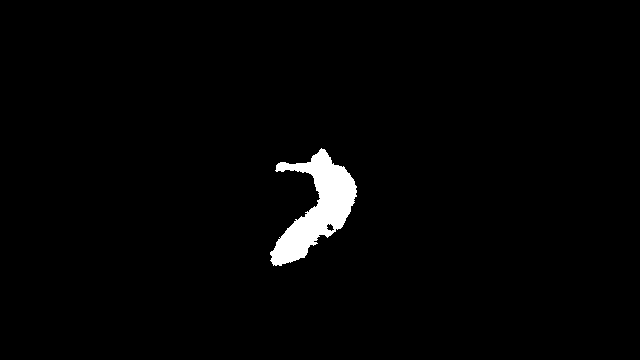} &\hspace{-4mm}
\includegraphics[width=0.16\linewidth]{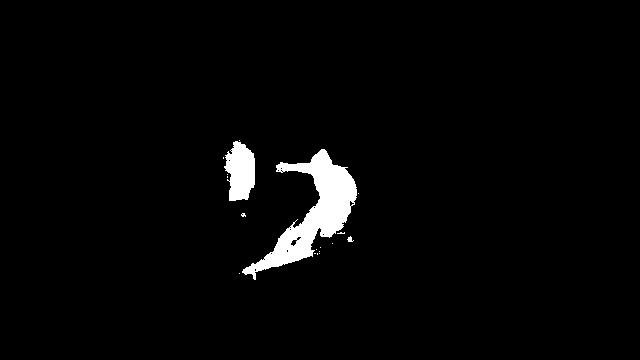} &\hspace{-4mm}
\includegraphics[width=0.16\linewidth]{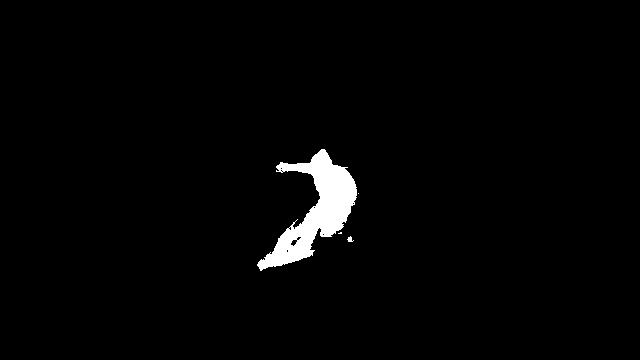} &\hspace{-4mm}
\includegraphics[width=0.16\linewidth]{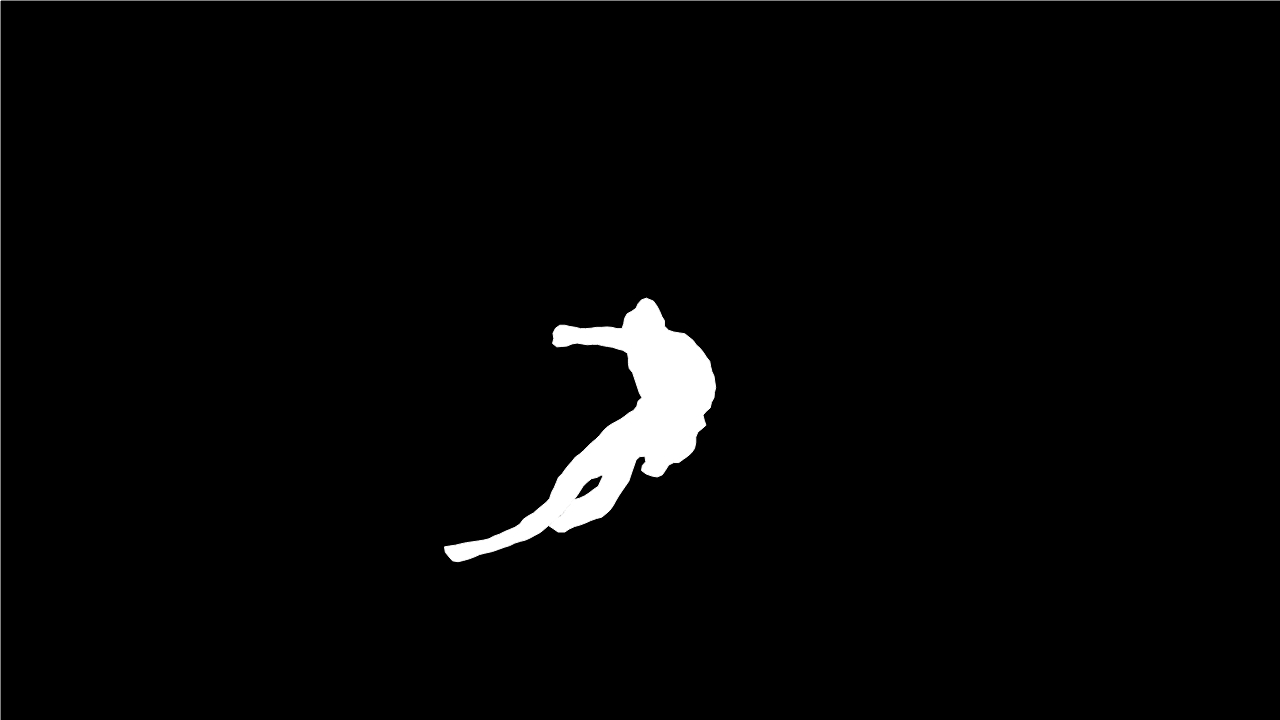} \\

\includegraphics[width=0.16\linewidth]{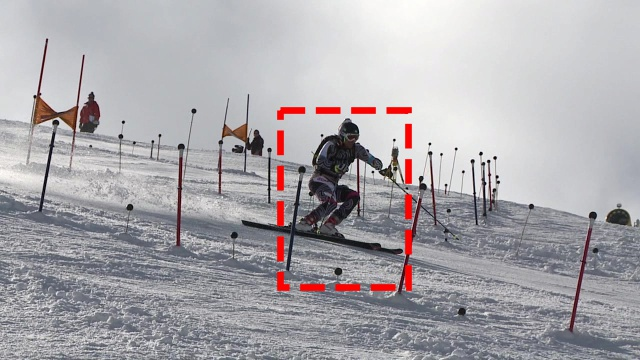} &\hspace{-4.0mm}
\includegraphics[width=0.16\linewidth]{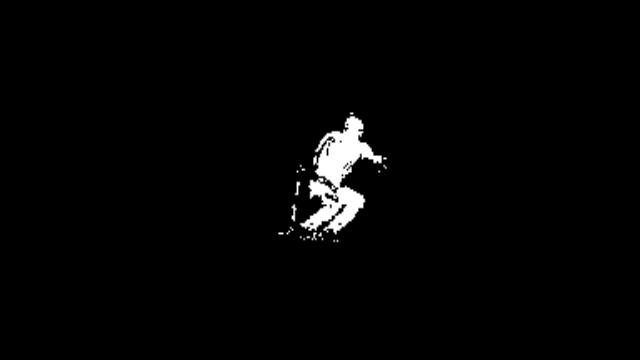} &\hspace{-4mm}
\includegraphics[width=0.16\linewidth]{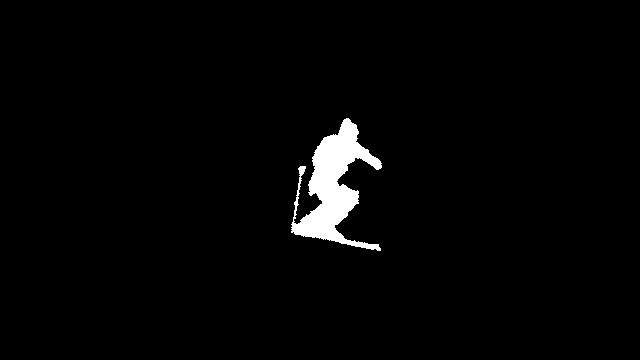} &\hspace{-4mm}
\includegraphics[width=0.16\linewidth]{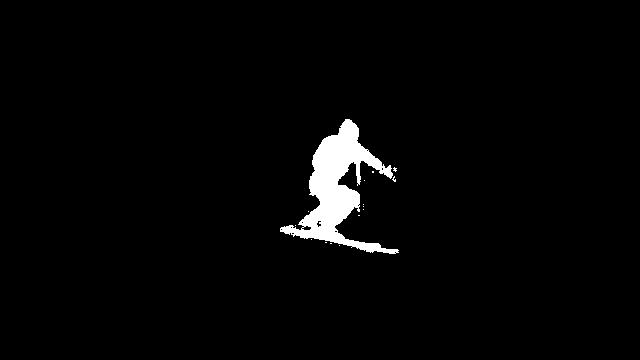} &\hspace{-4mm}
\includegraphics[width=0.16\linewidth]{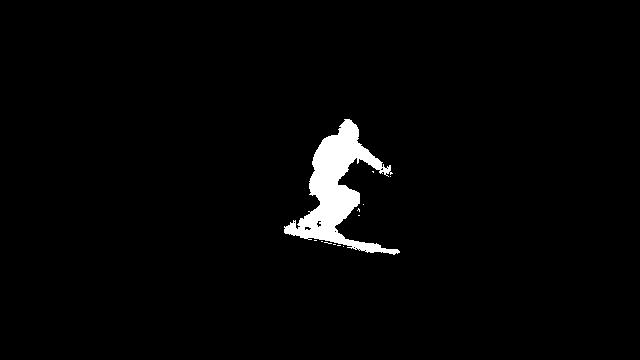} &\hspace{-4mm}
\includegraphics[width=0.16\linewidth]{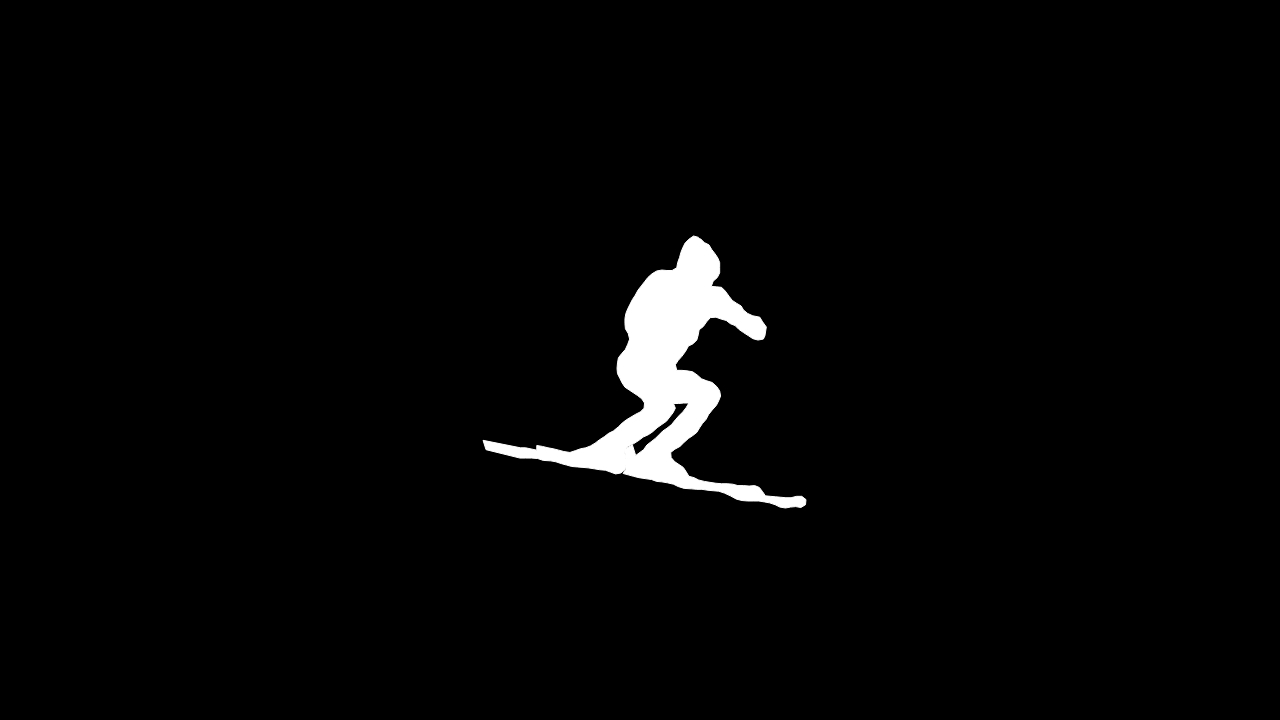} \\

\includegraphics[width=0.16\linewidth]{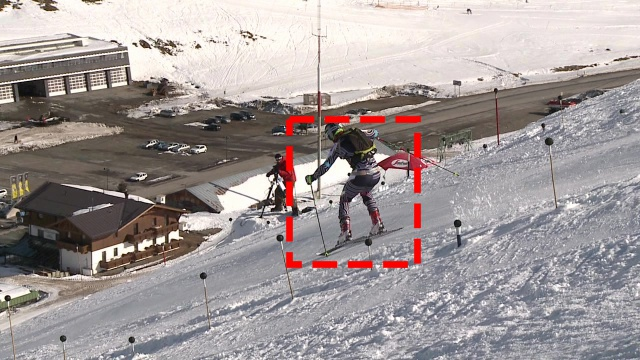} &\hspace{-4.0mm}
\includegraphics[width=0.16\linewidth]{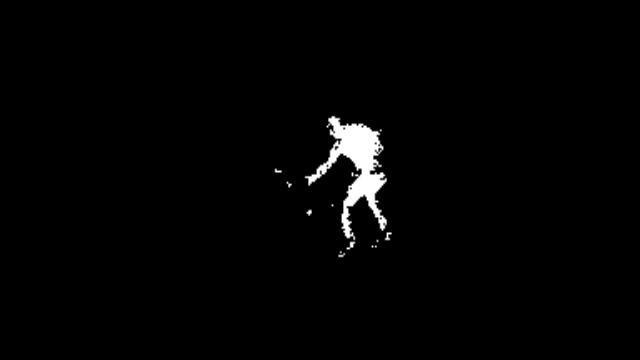} &\hspace{-4mm}
\includegraphics[width=0.16\linewidth]{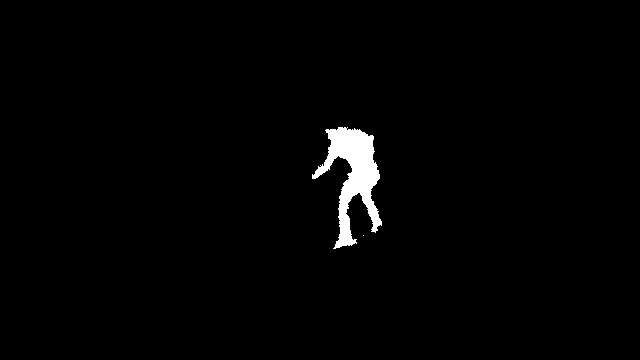} &\hspace{-4mm}
\includegraphics[width=0.16\linewidth]{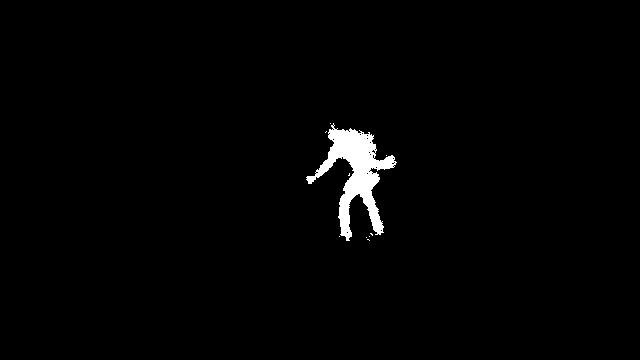} &\hspace{-4mm}
\includegraphics[width=0.16\linewidth]{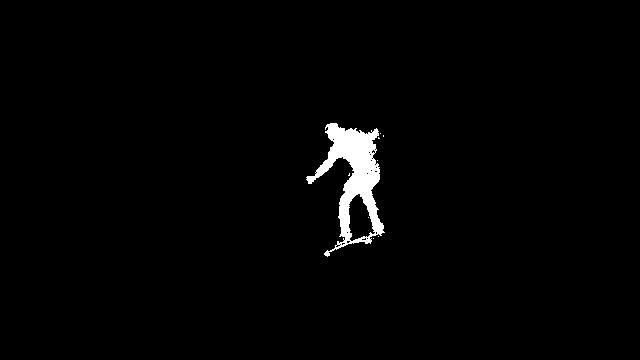} &\hspace{-4mm}
\includegraphics[width=0.16\linewidth]{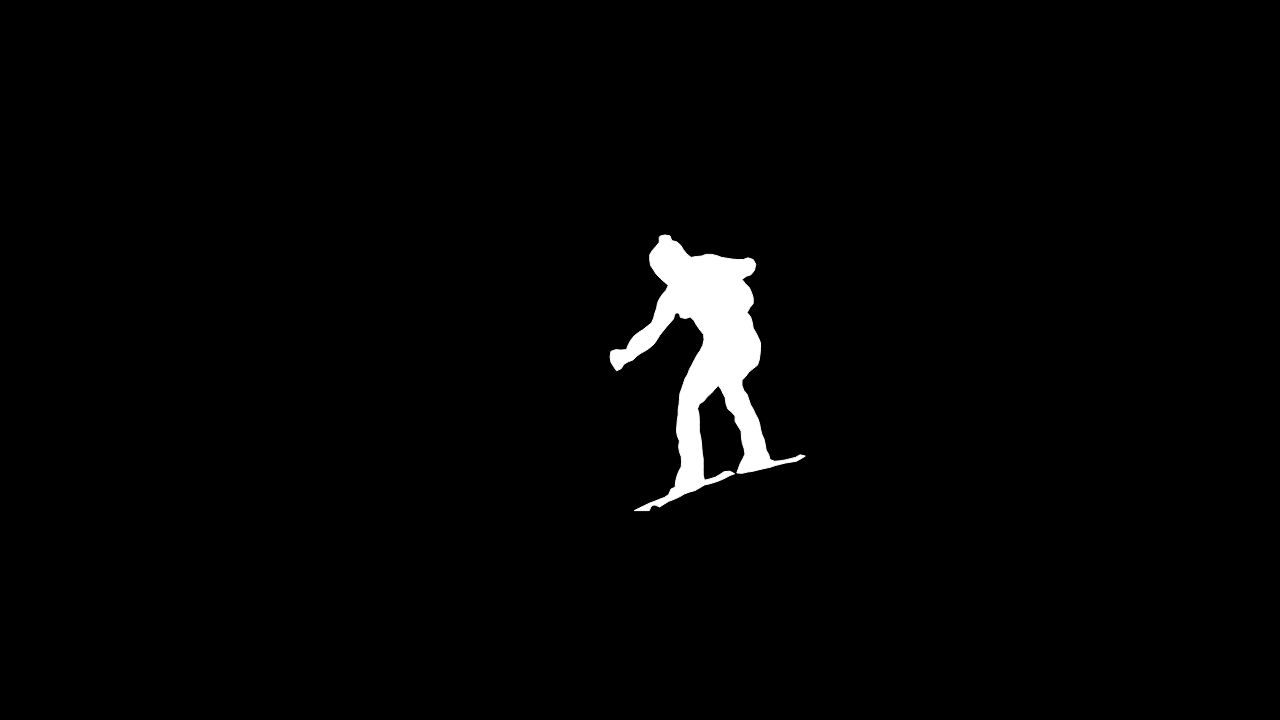} \\

\includegraphics[width=0.16\linewidth]{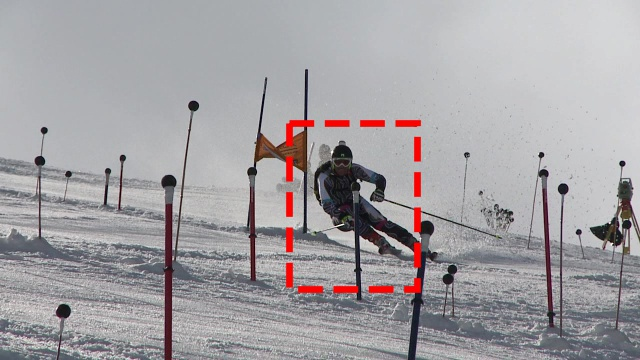} &\hspace{-4.0mm}
\includegraphics[width=0.16\linewidth]{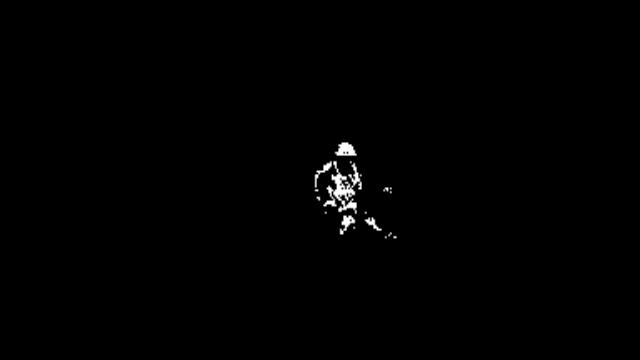} &\hspace{-4mm}
\includegraphics[width=0.16\linewidth]{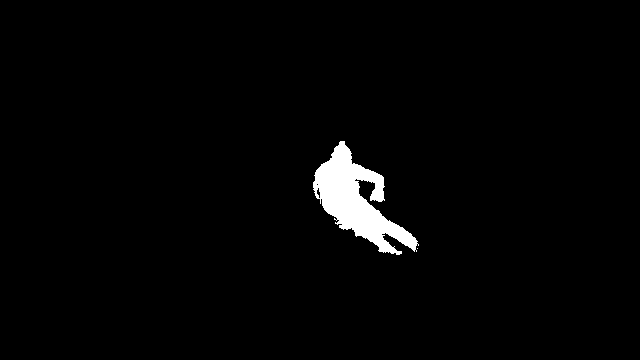} &\hspace{-4mm}
\includegraphics[width=0.16\linewidth]{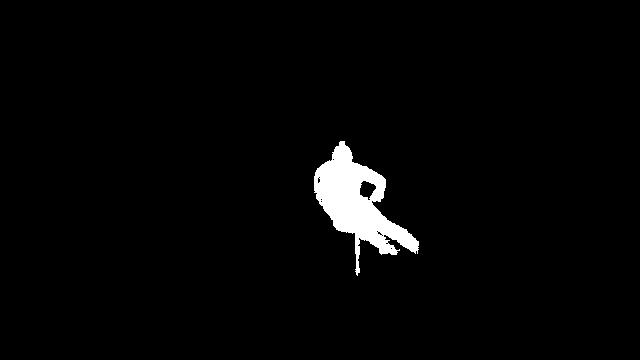} &\hspace{-4mm}
\includegraphics[width=0.16\linewidth]{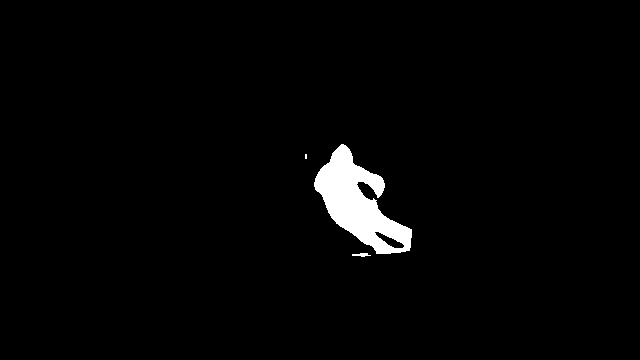} &\hspace{-4mm}
\includegraphics[width=0.16\linewidth]{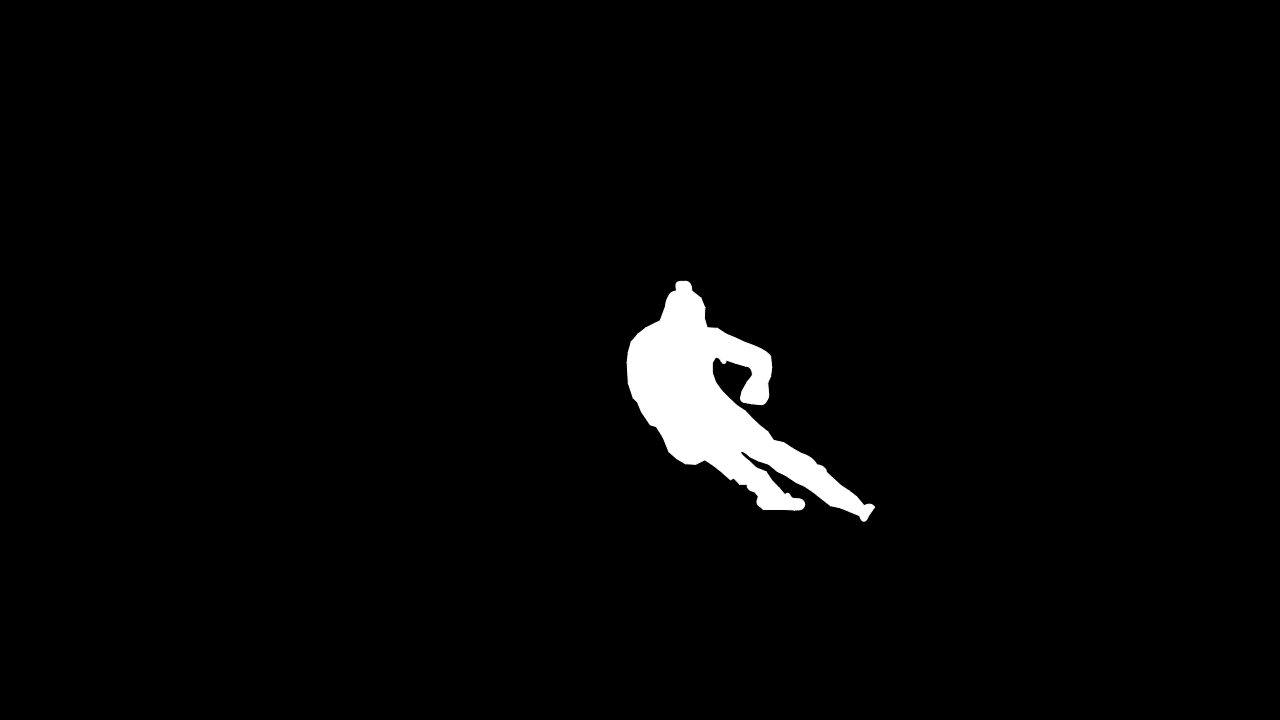}   \\

\\

  {\fontsize{8}{5}\selectfont  \hspace{-1mm}(a) Input/Ours detection}& \hspace{-1mm} {\fontsize{8}{5}\selectfont (b) Yang et al.~\cite{Yang19c}}&\hspace{-4mm} {\fontsize{8}{5}\selectfont (c) Koh et al.~\cite{Koh17b}} &\hspace{-4mm} {\fontsize{8}{5}\selectfont (d) Katircioglu et al.~\cite{Katircioglu20}}&\hspace{-4mm}   {\fontsize{8}{5}\selectfont (e) Ours}  &\hspace{-4mm}  {\fontsize{8}{5}\selectfont (f) GT }  \\ \\
  \end{tabular}}

  \caption{ \textbf{Qualitative results on the \ski{}.} (a) Input images with our predicted bounding box overlaid in red. (b) Segmentation mask prediction of~\cite{Yang19c}. (c) Segmentation mask prediction of~\cite{Koh17b}. (d) Segmentation mask prediction of~\cite{Katircioglu20} (e) Our segmentation mask prediction. (f) Ground truth segmentation mask. Note that, unlike our method,~\cite{Koh17b} and~\cite{Yang19c} use explicit temporal cues at inference time.}
  \label{fig:supp_ski_qual}
\end{figure*}
\clearpage

\begin{figure*}[hbt!]
  \centering
  {
  	\resizebox{\linewidth}{!}{

  \begin{tabular}{@{}ccccccc@{}}
   \includegraphics[width=0.137\linewidth]{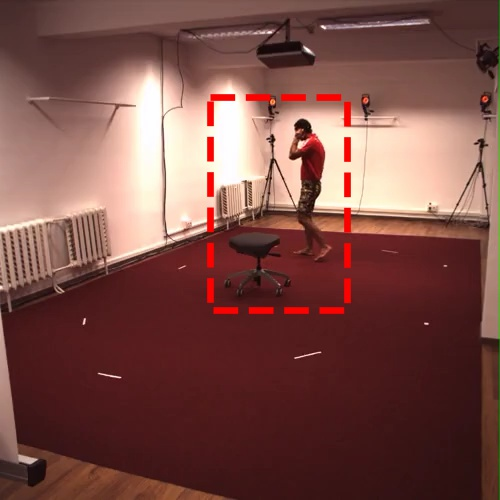}
   \includegraphics[width=0.137\linewidth]{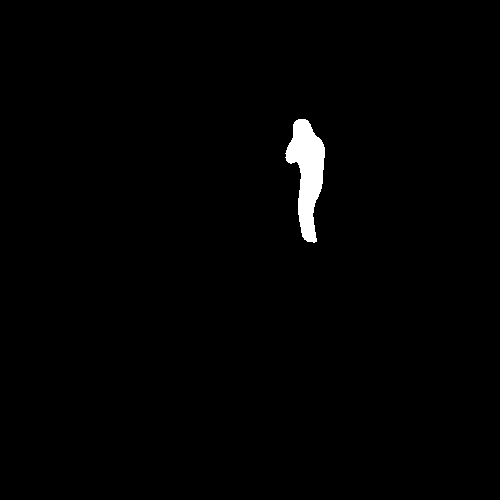}&
   
      \includegraphics[width=0.137\linewidth]{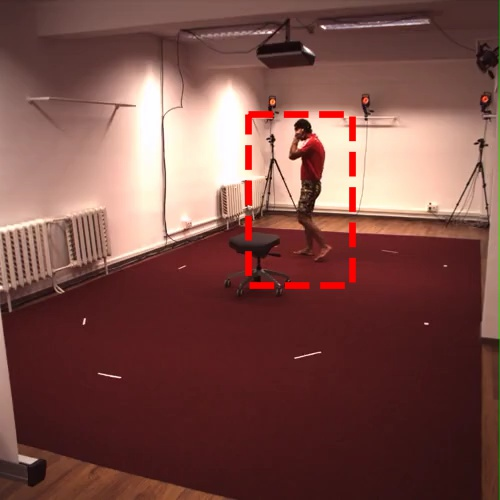} 
   \includegraphics[width=0.137\linewidth]{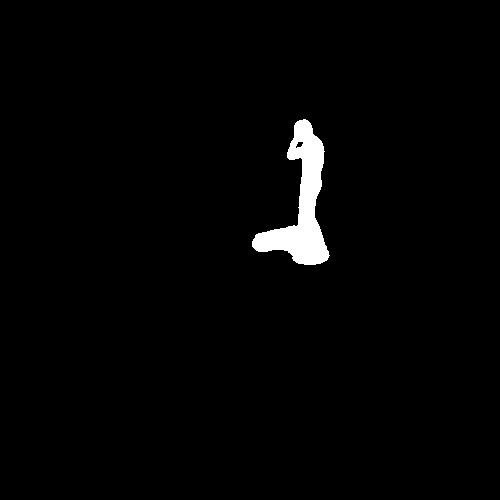} &

      \includegraphics[width=0.137\linewidth]{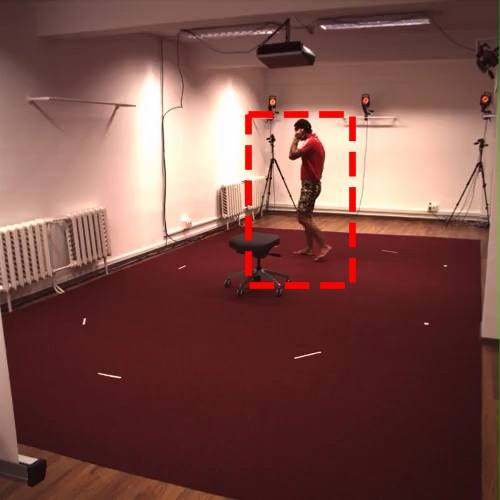} 
   \includegraphics[width=0.137\linewidth]{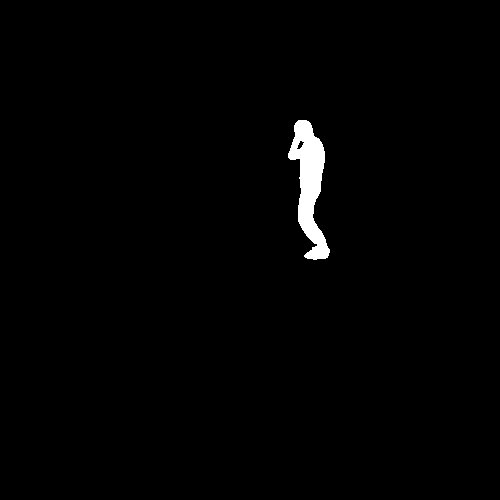} &

   \includegraphics[width=0.137\linewidth]{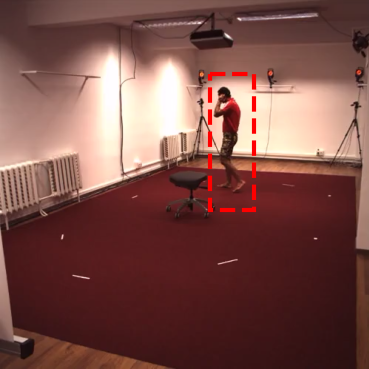} \\

   \includegraphics[width=0.137\linewidth]{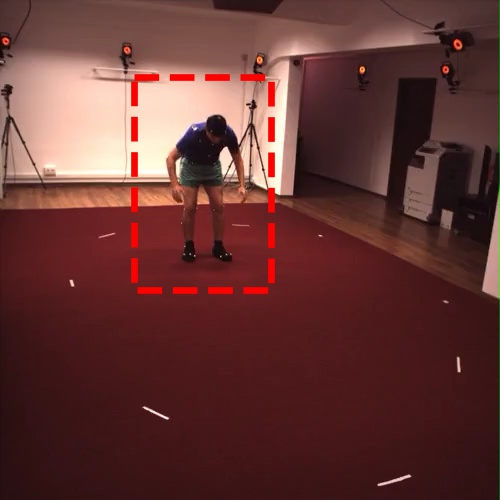}
   \includegraphics[width=0.137\linewidth]{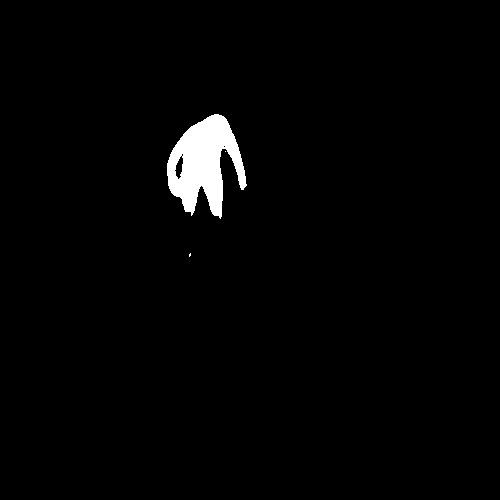}&
   
   \includegraphics[width=0.137\linewidth]{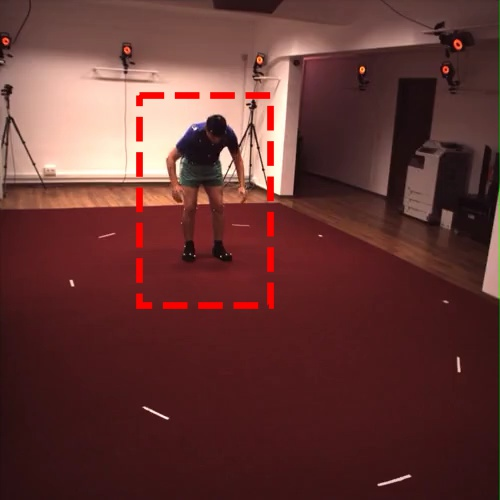} 
   \includegraphics[width=0.137\linewidth]{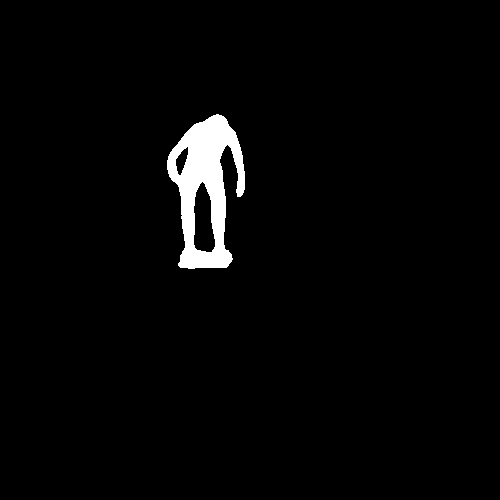} &

   \includegraphics[width=0.137\linewidth]{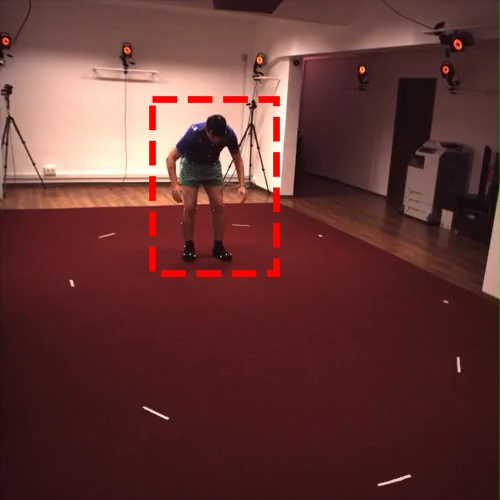} 
   \includegraphics[width=0.137\linewidth]{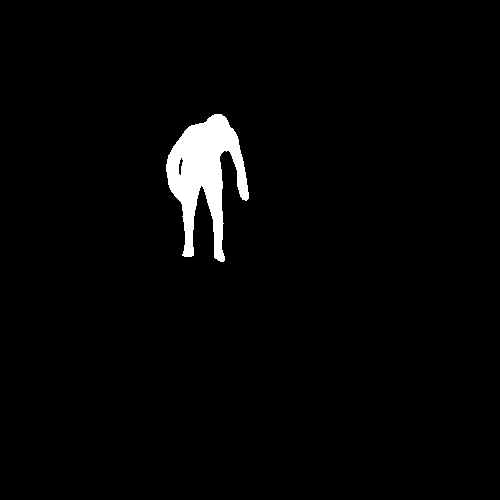} &

   \includegraphics[width=0.137\linewidth]{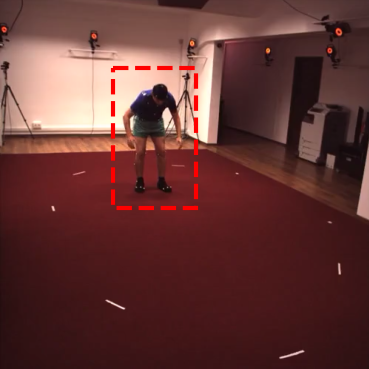} \\

 \includegraphics[width=0.137\linewidth]{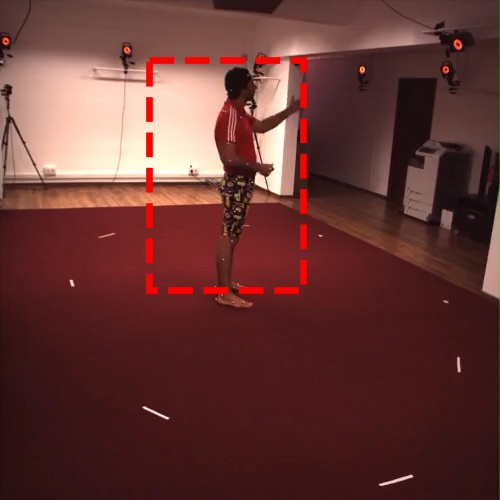}
\includegraphics[width=0.137\linewidth]{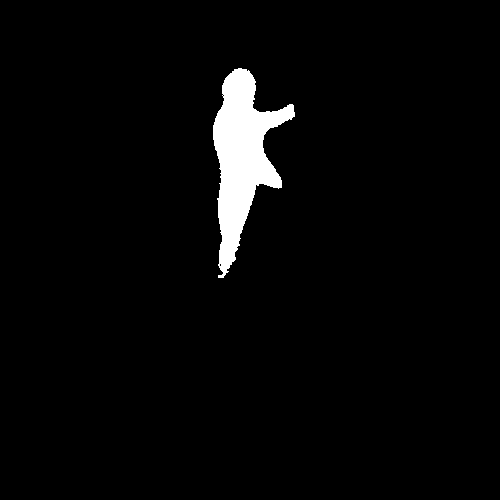}&

\includegraphics[width=0.137\linewidth]{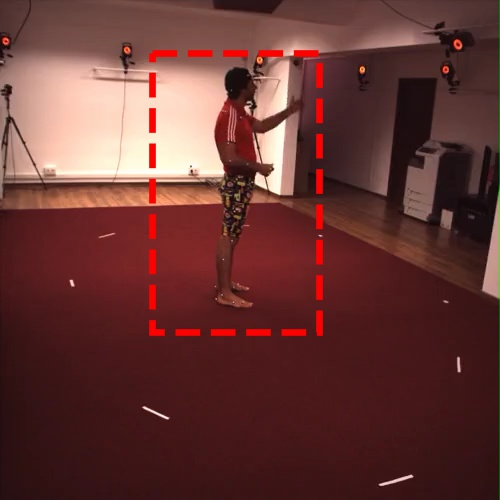} 
\includegraphics[width=0.137\linewidth]{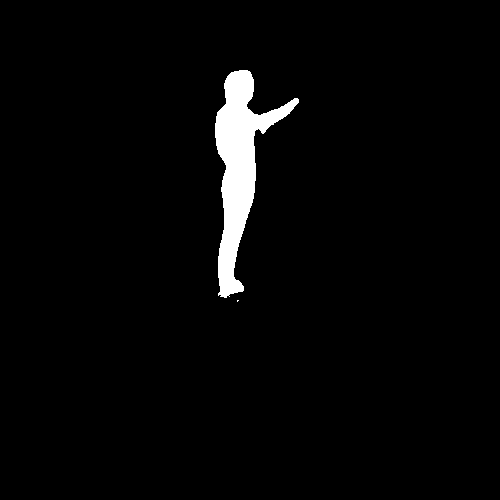} &

\includegraphics[width=0.137\linewidth]{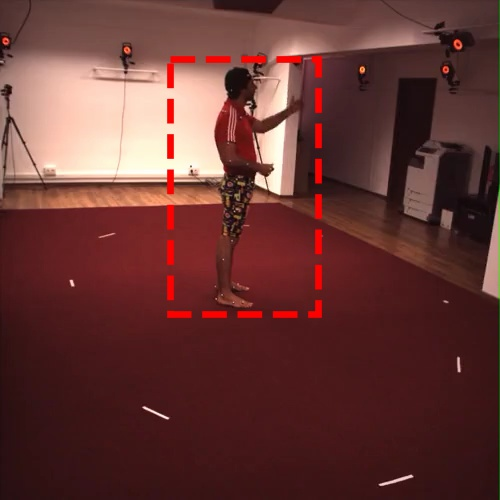} 
\includegraphics[width=0.137\linewidth]{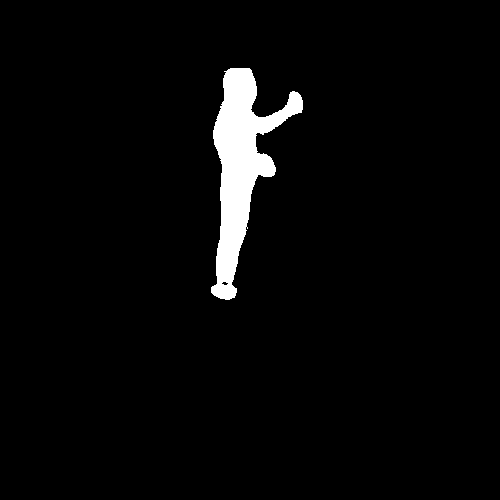} &

\includegraphics[width=0.137\linewidth]{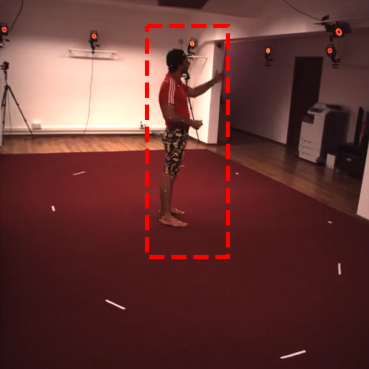} \\

\includegraphics[width=0.137\linewidth]{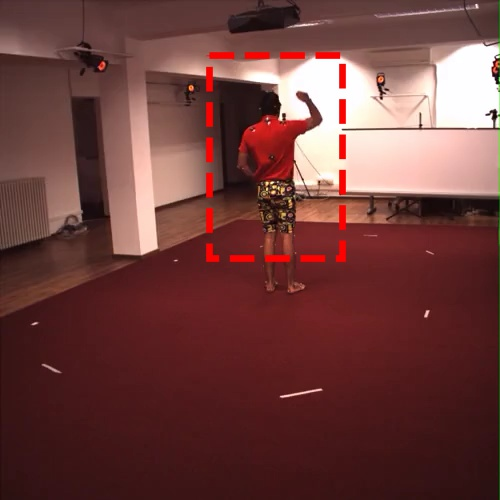}
\includegraphics[width=0.137\linewidth]{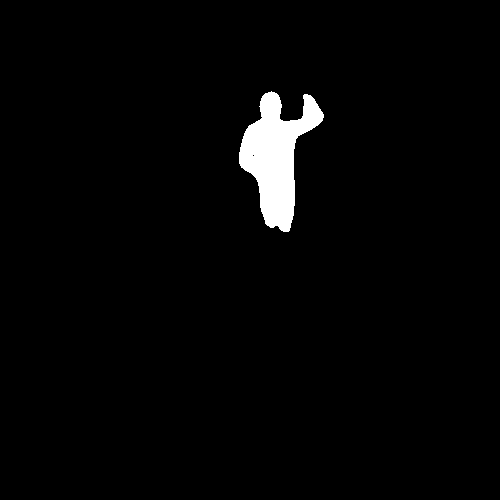} &

\includegraphics[width=0.137\linewidth]{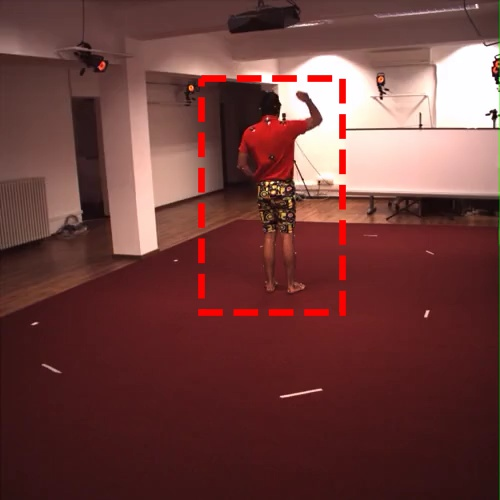}
\includegraphics[width=0.137\linewidth]{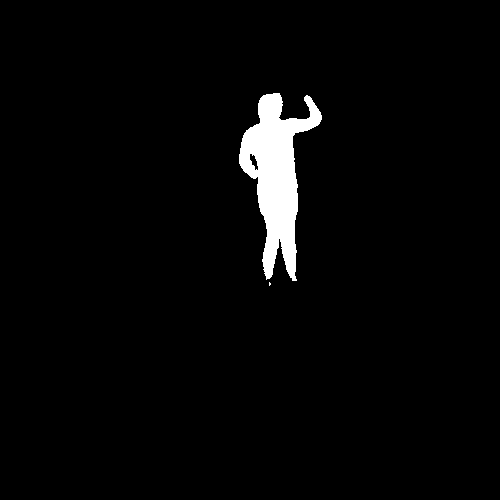}&

\includegraphics[width=0.137\linewidth]{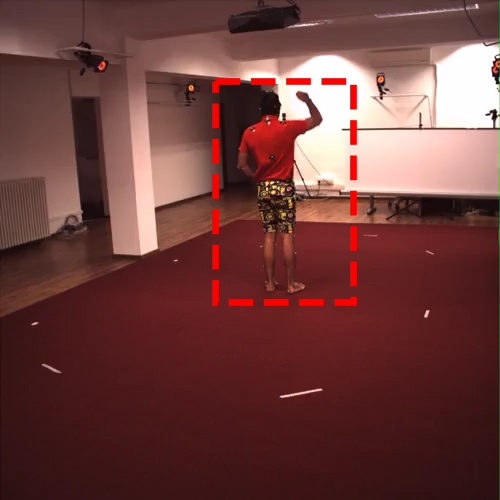}
\includegraphics[width=0.137\linewidth]{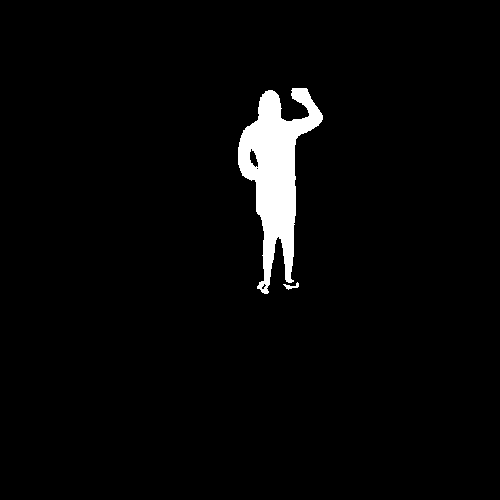}&

\includegraphics[width=0.137\linewidth]{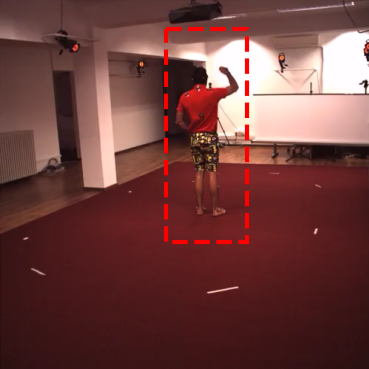} \\

\includegraphics[width=0.137\linewidth]{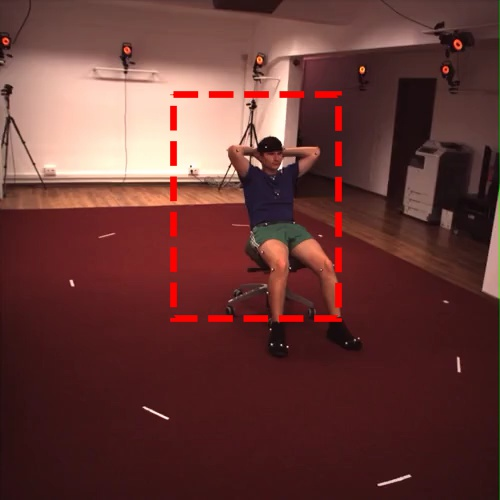}
\includegraphics[width=0.137\linewidth]{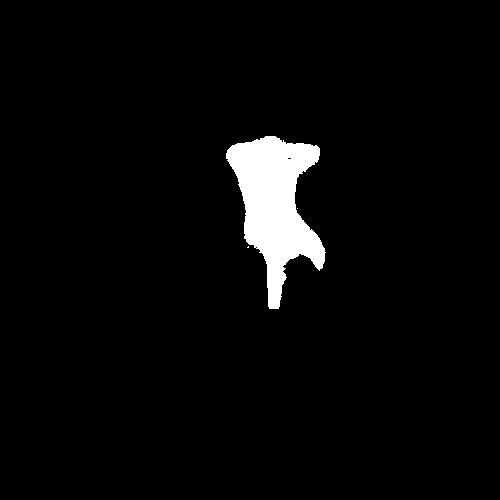} &

\includegraphics[width=0.137\linewidth]{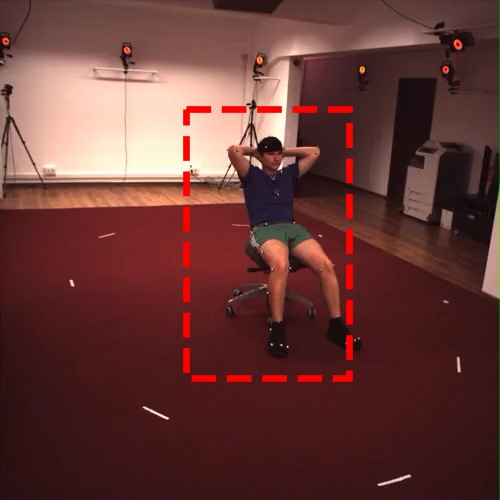}
\includegraphics[width=0.137\linewidth]{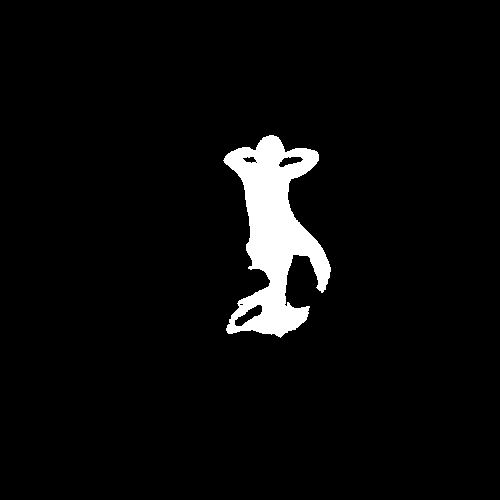}&

\includegraphics[width=0.137\linewidth]{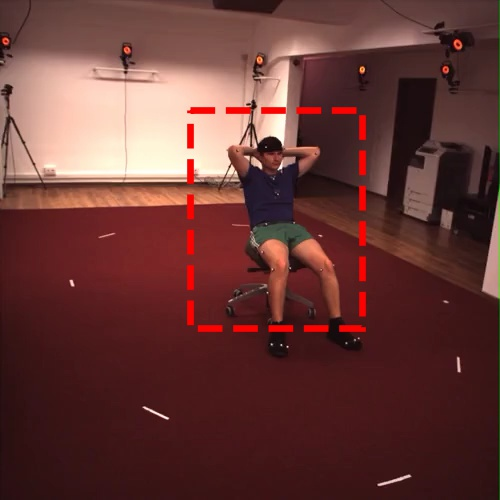}
\includegraphics[width=0.137\linewidth]{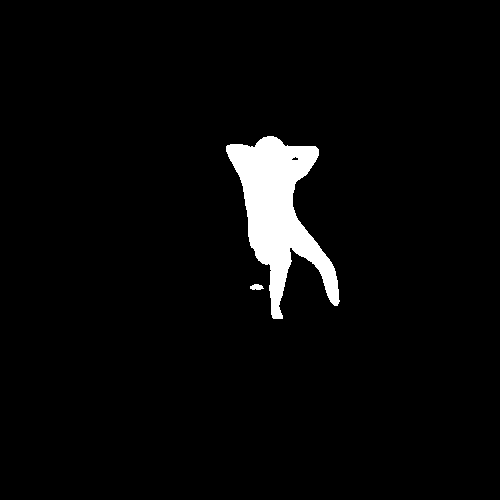}&

\includegraphics[width=0.137\linewidth]{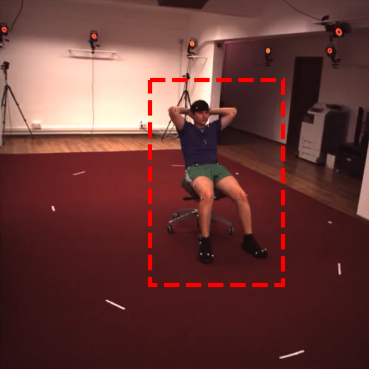} \\

\includegraphics[width=0.137\linewidth]{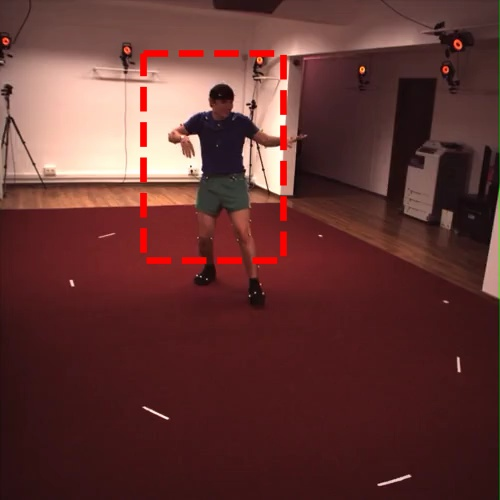}
\includegraphics[width=0.137\linewidth]{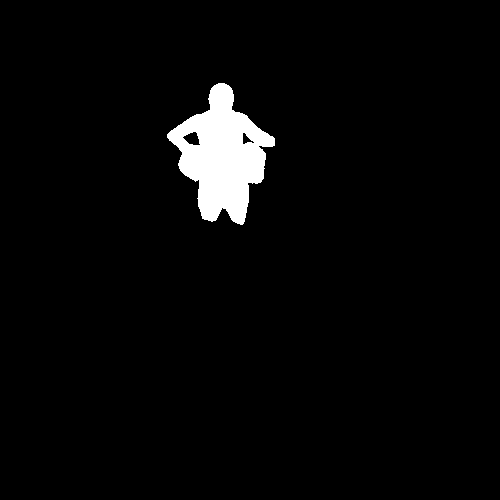} &

\includegraphics[width=0.137\linewidth]{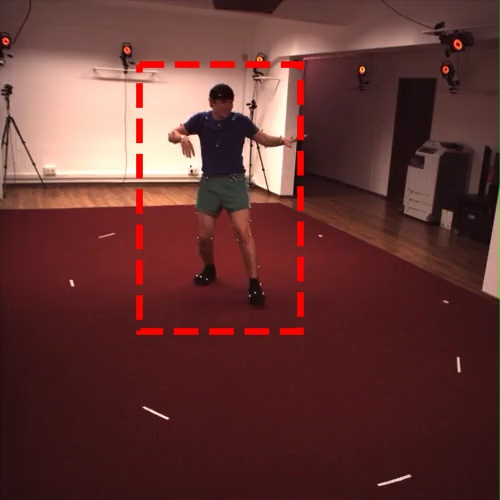}
\includegraphics[width=0.137\linewidth]{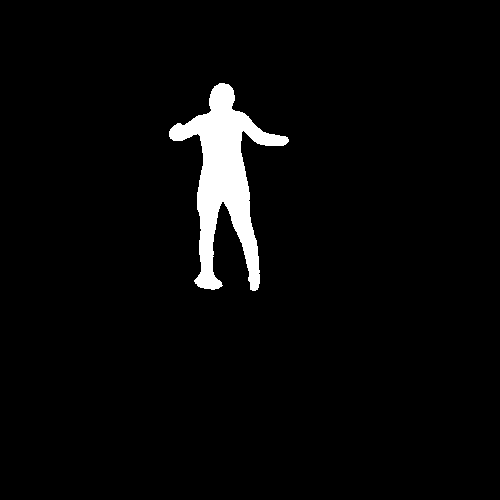}&

\includegraphics[width=0.137\linewidth]{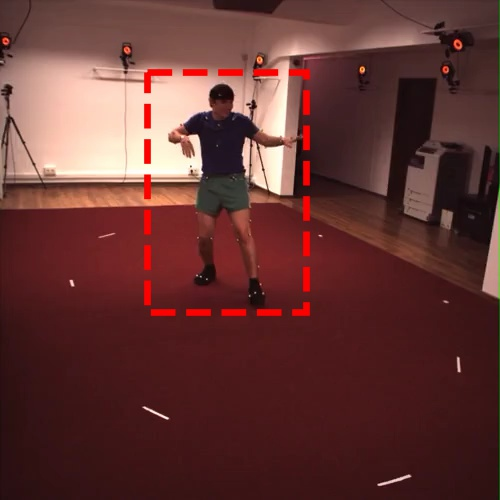}
\includegraphics[width=0.137\linewidth]{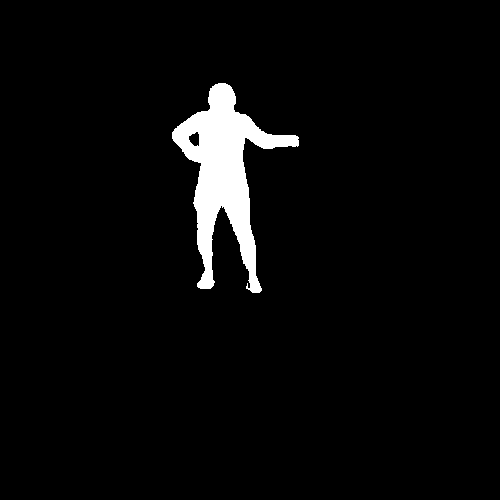}&

\includegraphics[width=0.137\linewidth]{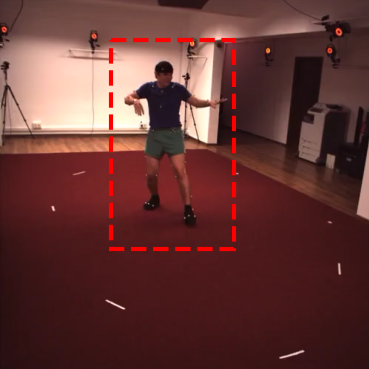} \\

\includegraphics[width=0.137\linewidth]{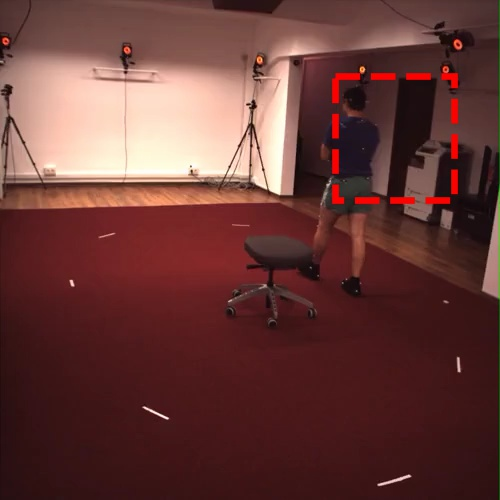}
\includegraphics[width=0.137\linewidth]{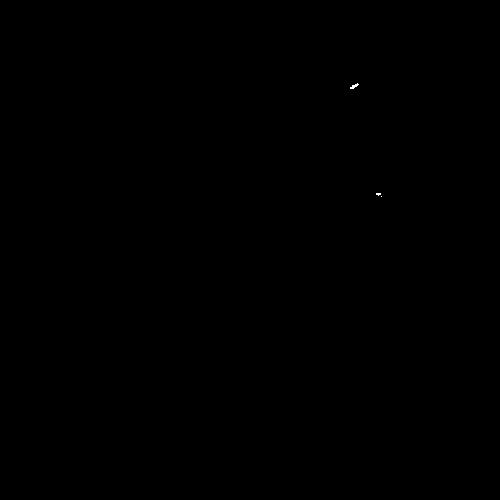} &

\includegraphics[width=0.137\linewidth]{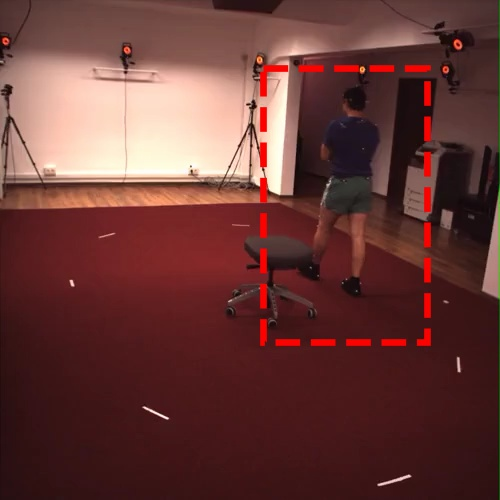}
\includegraphics[width=0.137\linewidth]{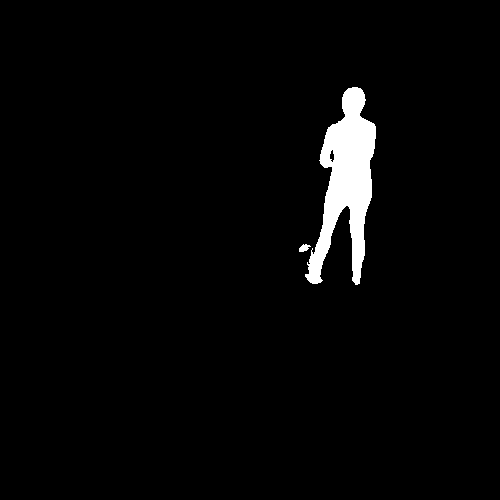}&

\includegraphics[width=0.137\linewidth]{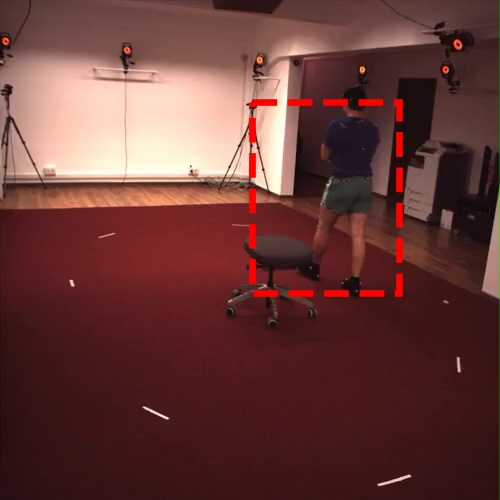}
\includegraphics[width=0.137\linewidth]{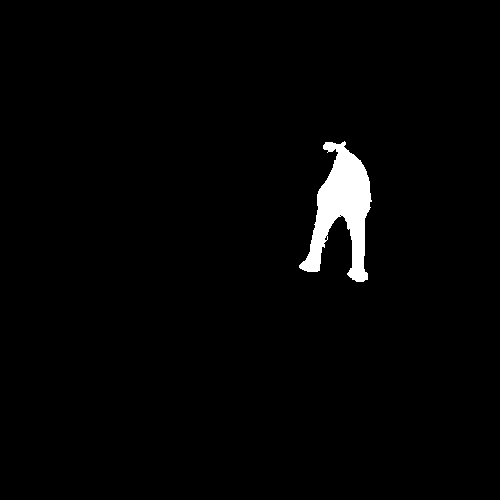}&

\includegraphics[width=0.137\linewidth]{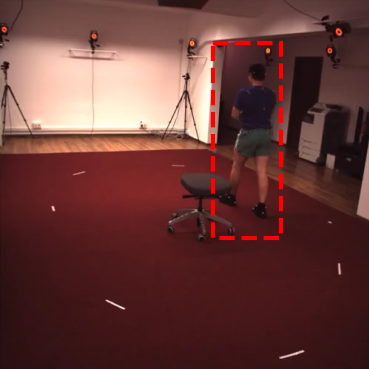} \\

\includegraphics[width=0.137\linewidth]{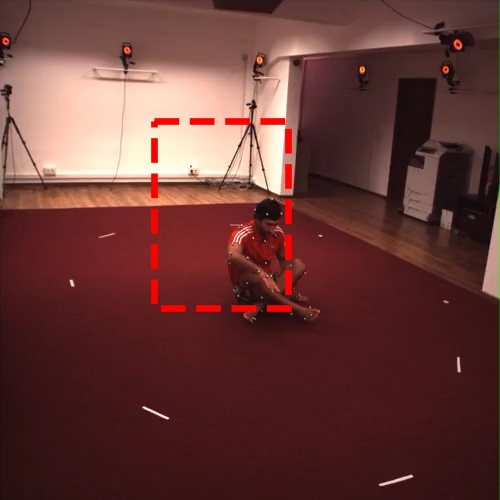}
\includegraphics[width=0.137\linewidth]{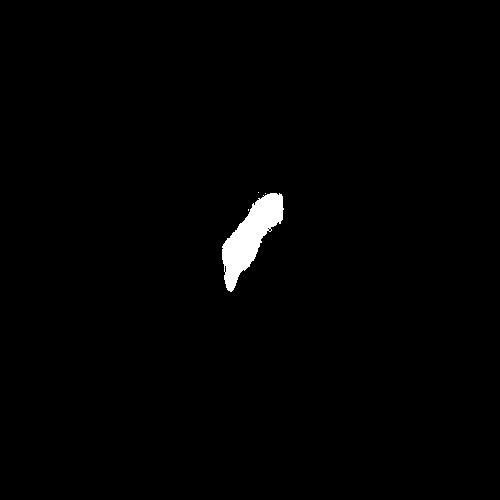} &

\includegraphics[width=0.137\linewidth]{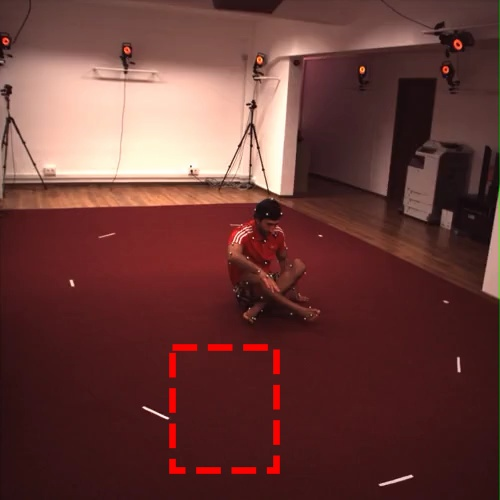}
\includegraphics[width=0.137\linewidth]{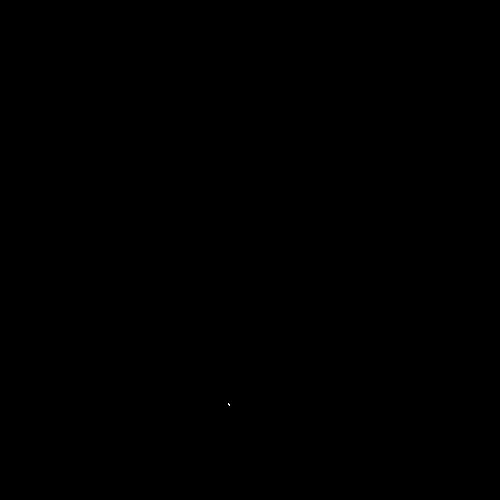}&

\includegraphics[width=0.137\linewidth]{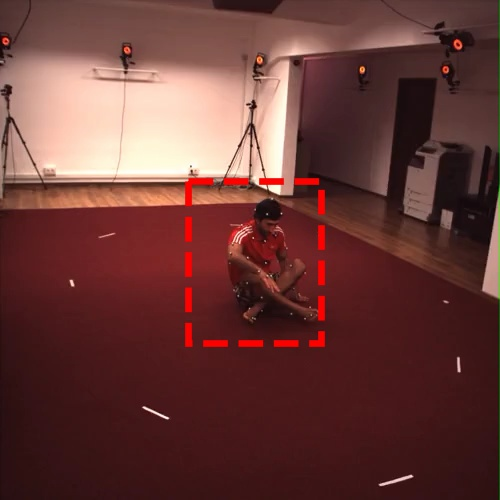}
\includegraphics[width=0.137\linewidth]{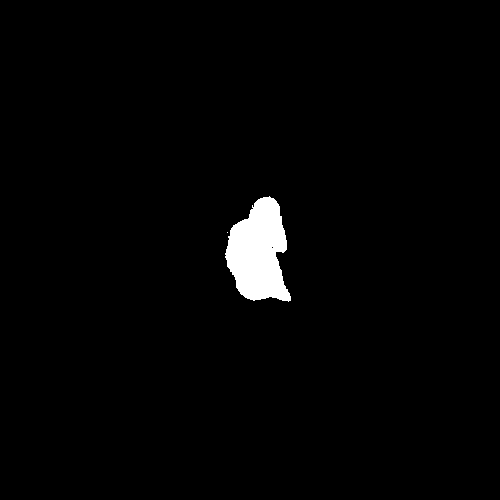}&

\includegraphics[width=0.137\linewidth]{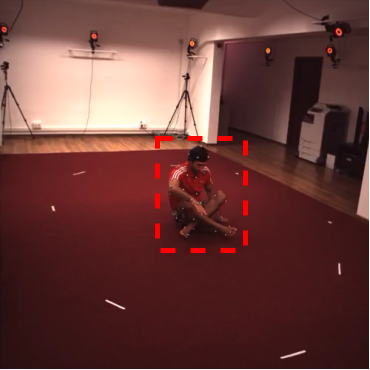} \\

\includegraphics[width=0.137\linewidth]{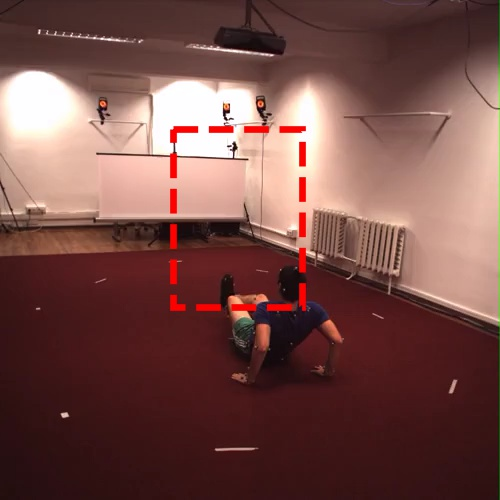}
\includegraphics[width=0.137\linewidth]{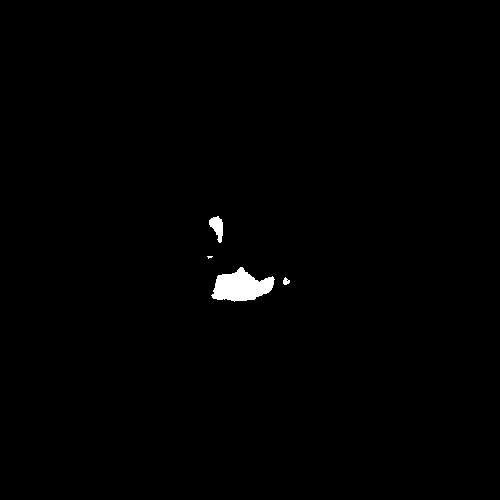} &

\includegraphics[width=0.137\linewidth]{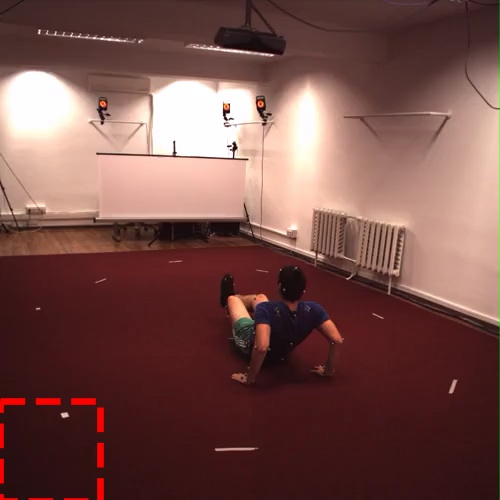}
\includegraphics[width=0.137\linewidth]{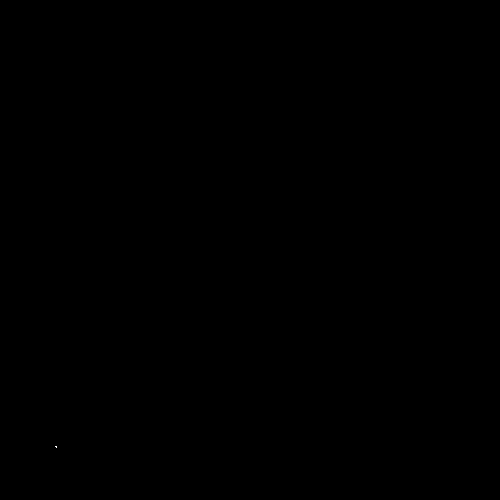}&

\includegraphics[width=0.137\linewidth]{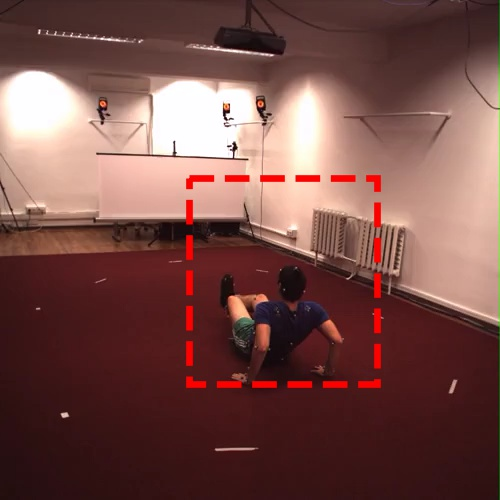}
\includegraphics[width=0.137\linewidth]{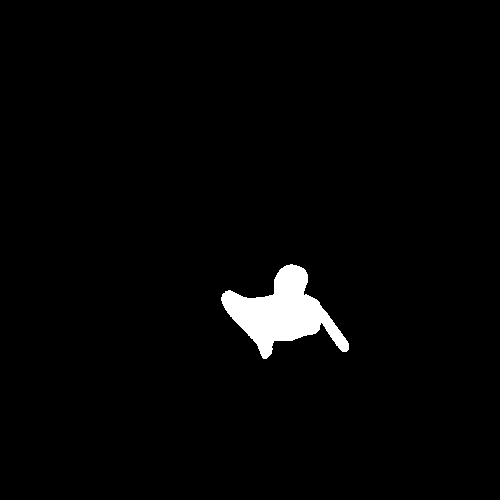}&

\includegraphics[width=0.137\linewidth]{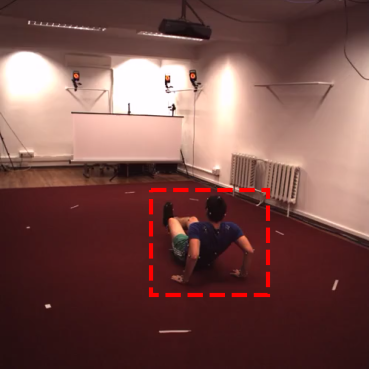} \\

    \includegraphics[width=0.137\linewidth]{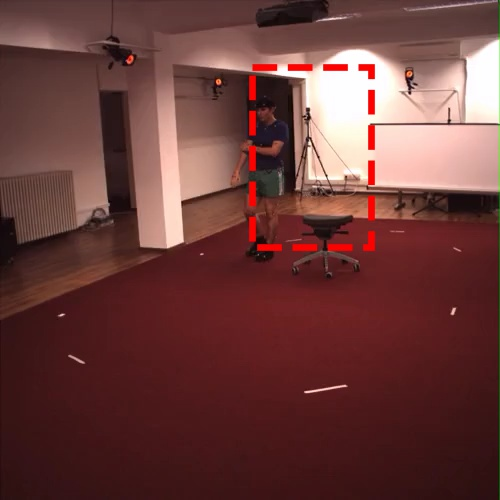}
   \includegraphics[width=0.137\linewidth]{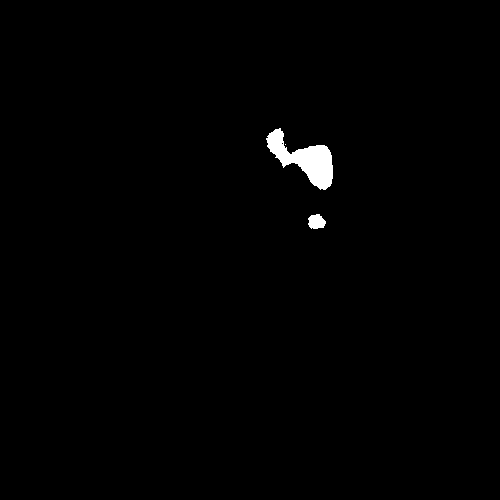}&
   
   \includegraphics[width=0.137\linewidth]{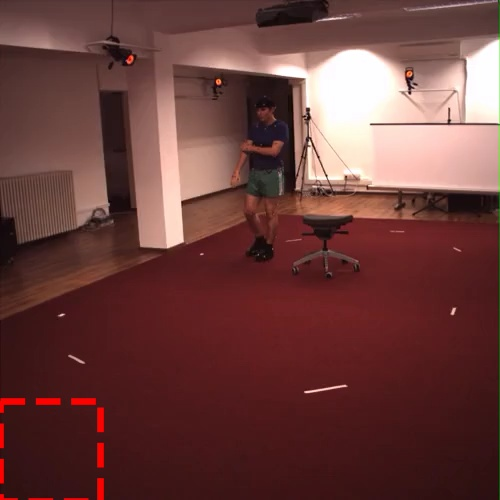} 
   \includegraphics[width=0.137\linewidth]{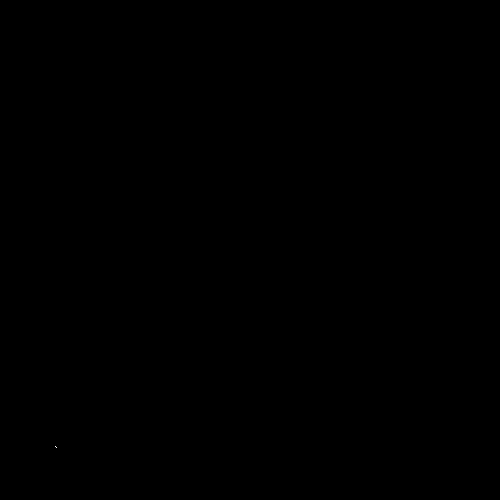} &

   \includegraphics[width=0.137\linewidth]{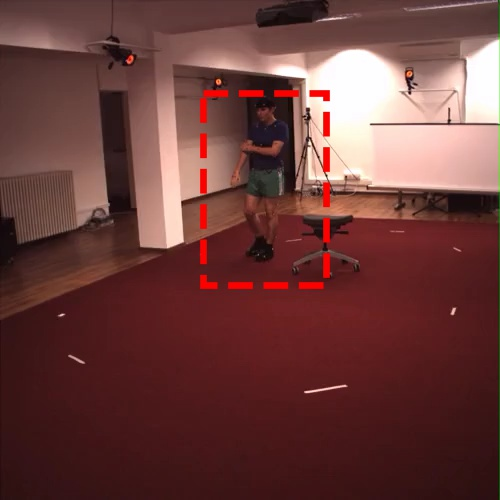} 
   \includegraphics[width=0.137\linewidth]{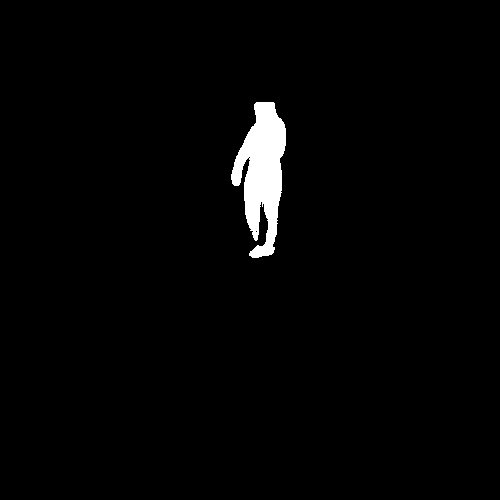} &

   \includegraphics[width=0.137\linewidth]{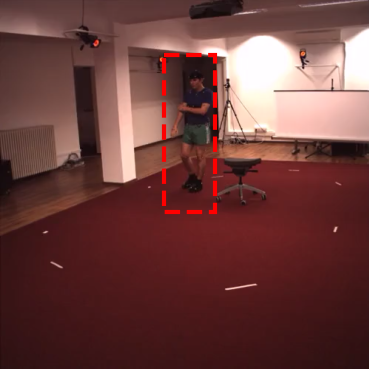} \\

 \\

{\fontsize{10}{5}\selectfont  (a)~Katircioglu et al.~\cite{Katircioglu20}}& {\fontsize{10}{5}\selectfont(b) Rhodin et al.~\cite{Rhodin19a}} &  {\fontsize{10}{5}\selectfont (c) Ours}  & {\fontsize{10}{5}\selectfont (d) GT }  \\ \\
  \end{tabular}}
}
  \caption{\textbf{Qualitative results on the {\human} dataset.} (a) The detection and segmentation mask results of Katircioglu et al.~\cite{Katircioglu20} trained and tested on single images. (b) The results of~\cite{Rhodin19a} trained with a pair of camera views and tested on single images. (c) Our predictions obtained from the model trained with the 4-cam multi-view consistency and tested on single images. (d) Ground truth.}
  \label{fig:supp_h36m_qual}
\end{figure*}
\clearpage

% !TEX root = ../top.tex
% !TEX spellcheck = en-US

\begin{figure*}[hbt!]
  \centering
  {
  	\resizebox{\linewidth}{!}{

  \begin{tabular}{@{}ccccc@{}}
   \includegraphics[width=0.45\linewidth]{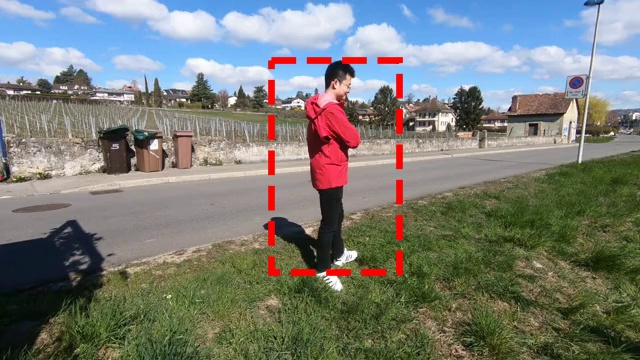}
   \includegraphics[width=0.45\linewidth]{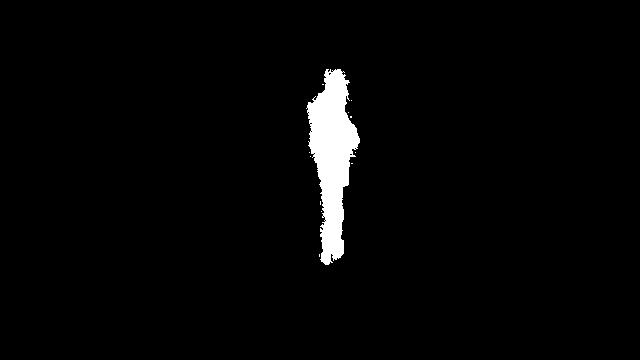}&
   
      \includegraphics[width=0.45\linewidth]{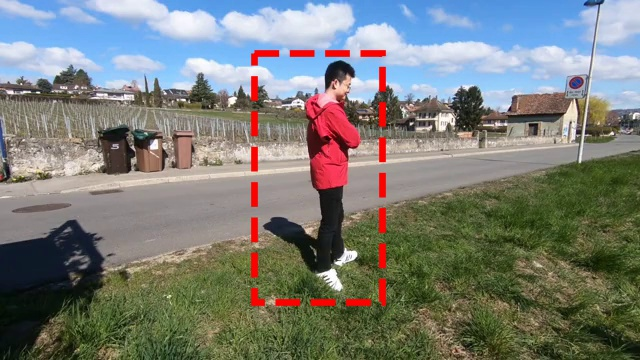} 
   \includegraphics[width=0.45\linewidth]{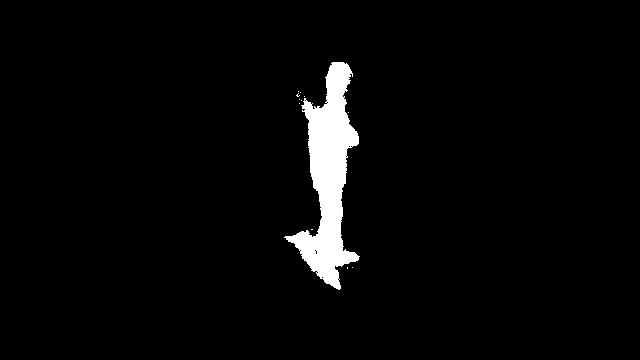} &
   
   \includegraphics[width=0.45\linewidth]{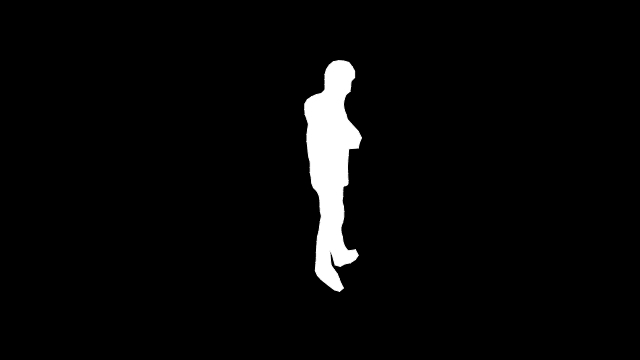} \\

    \includegraphics[width=0.45\linewidth]{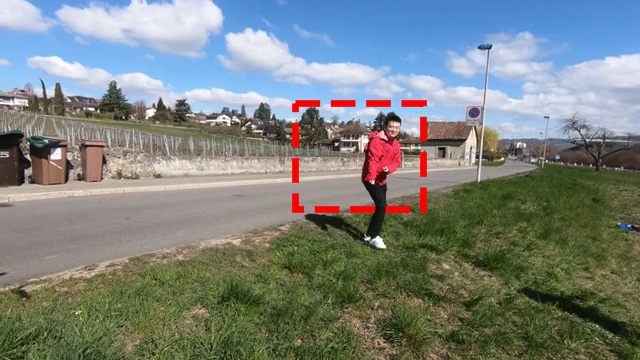}
   \includegraphics[width=0.45\linewidth]{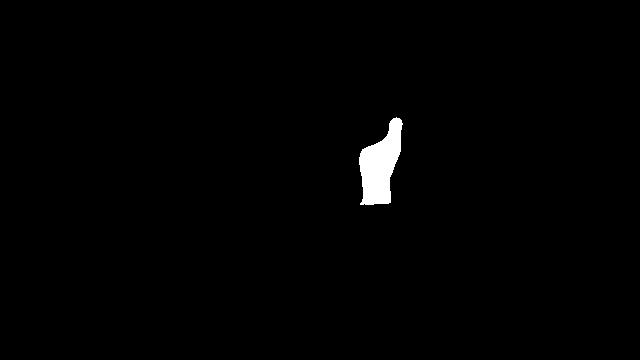}&
   
   \includegraphics[width=0.45\linewidth]{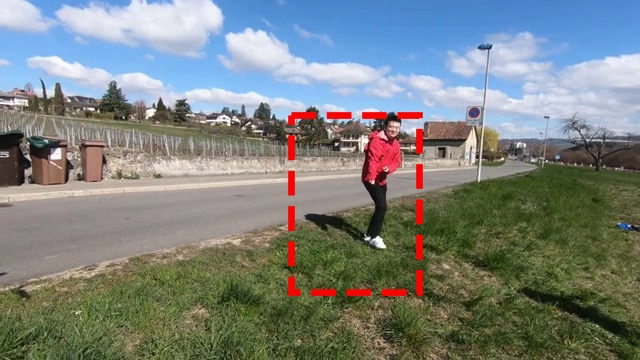} 
   \includegraphics[width=0.45\linewidth]{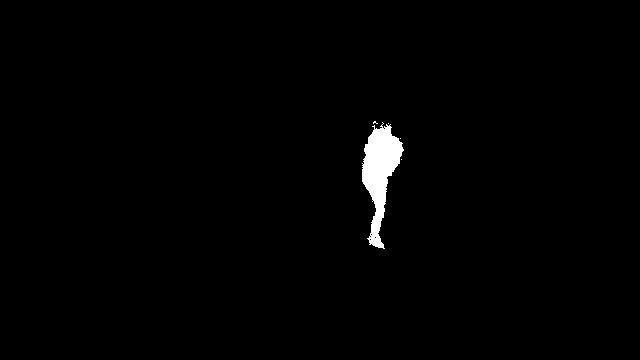} &
   
   \includegraphics[width=0.45\linewidth]{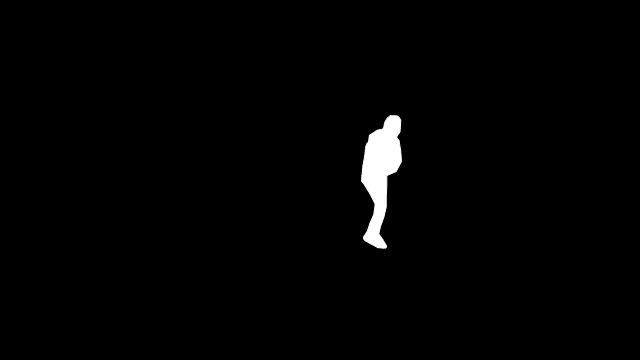} \\

    \includegraphics[width=0.45\linewidth]{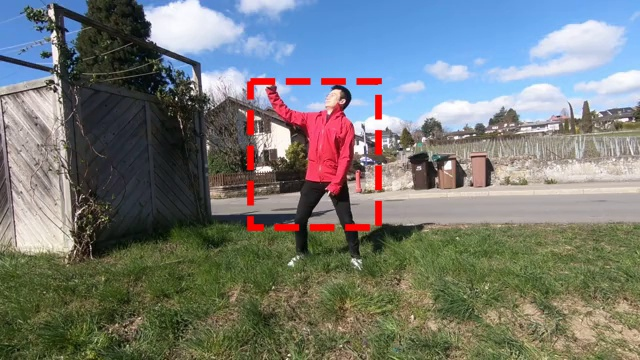}
   \includegraphics[width=0.45\linewidth]{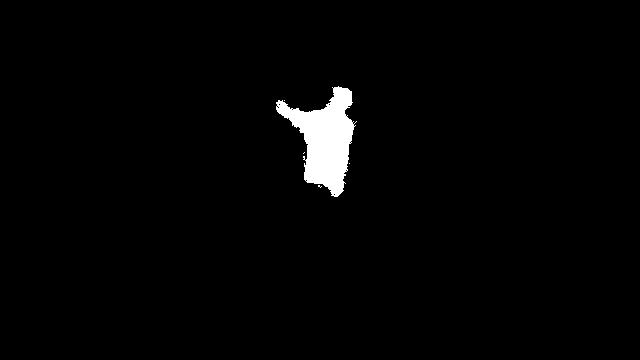}&
   
   \includegraphics[width=0.45\linewidth]{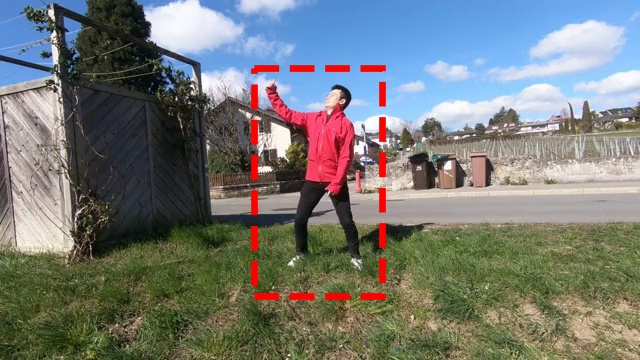} 
   \includegraphics[width=0.45\linewidth]{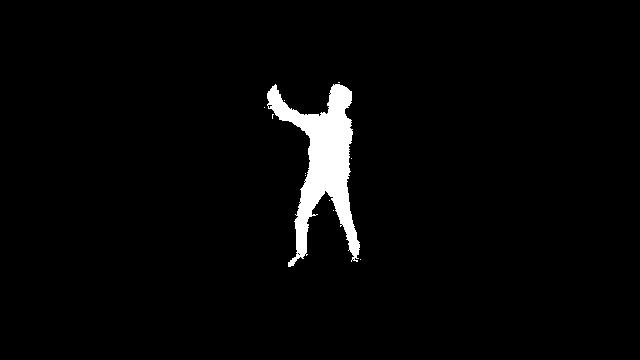} &
   
   \includegraphics[width=0.45\linewidth]{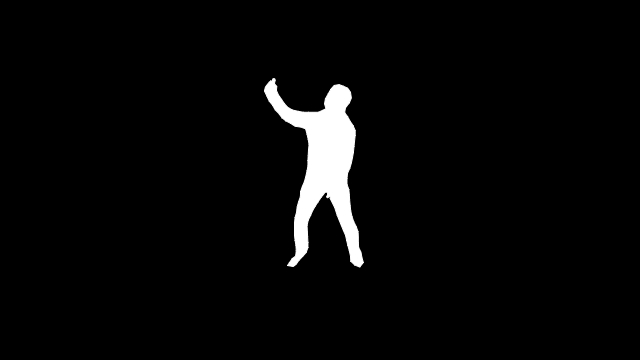} \\

    \includegraphics[width=0.45\linewidth]{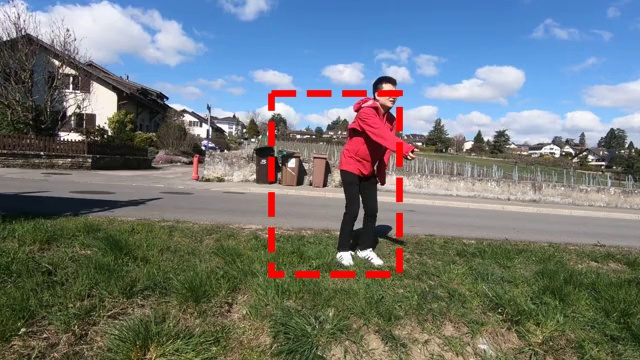}
   \includegraphics[width=0.45\linewidth]{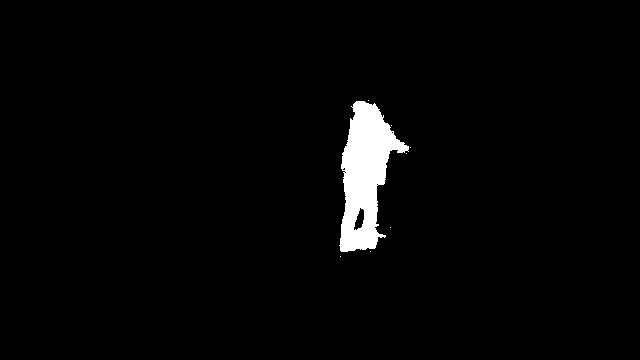}&
   
   \includegraphics[width=0.45\linewidth]{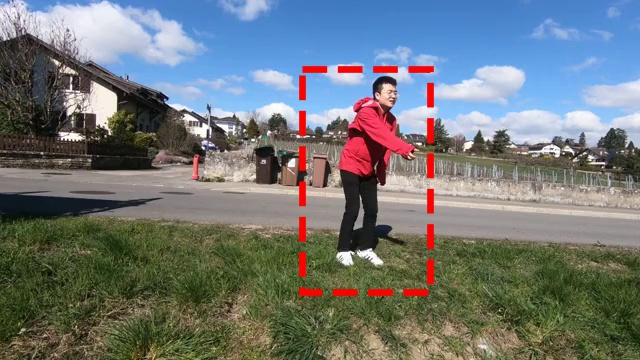} 
   \includegraphics[width=0.45\linewidth]{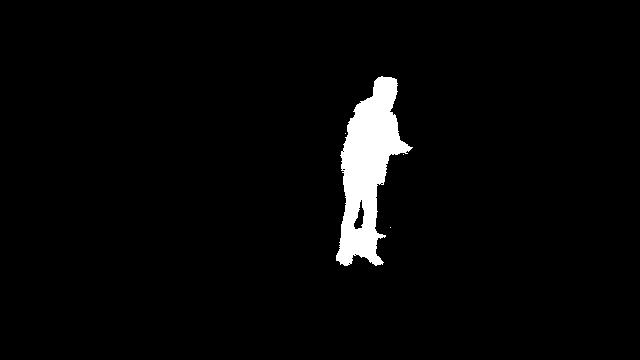} &
   
   \includegraphics[width=0.45\linewidth]{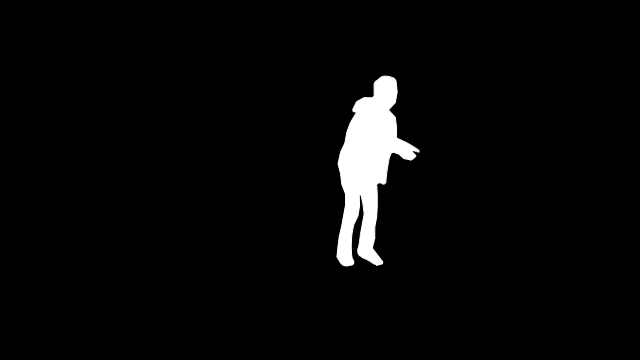} \\

    \includegraphics[width=0.45\linewidth]{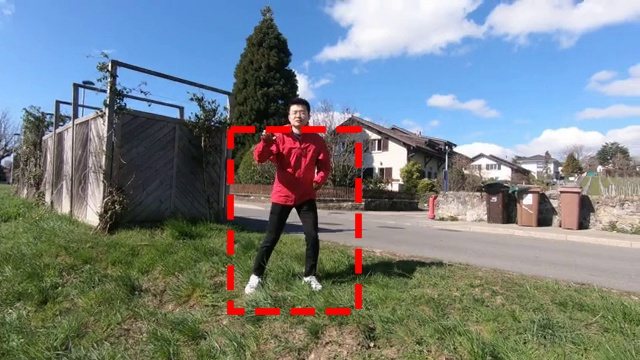}
   \includegraphics[width=0.45\linewidth]{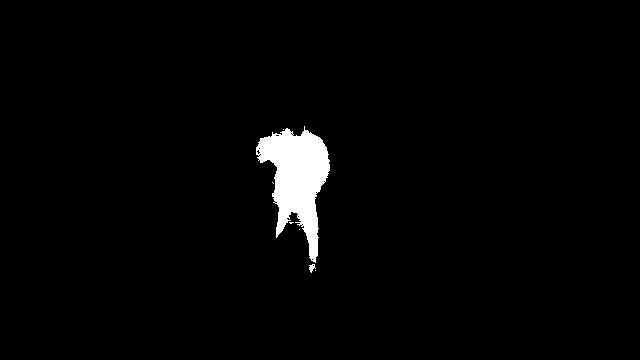}&
   
   \includegraphics[width=0.45\linewidth]{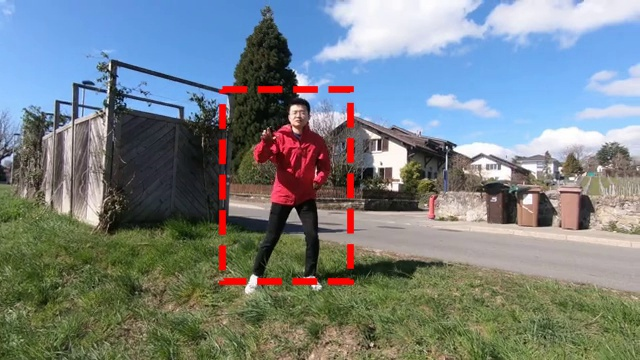} 
   \includegraphics[width=0.45\linewidth]{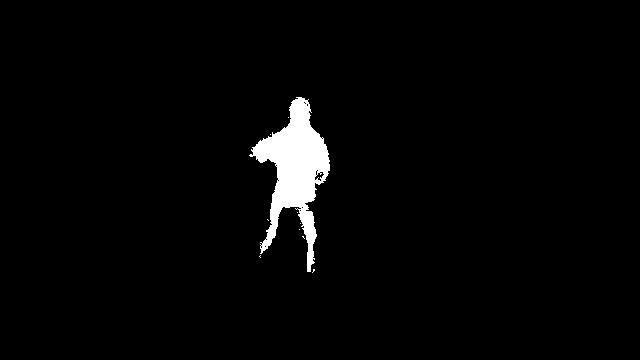} &
   
   \includegraphics[width=0.45\linewidth]{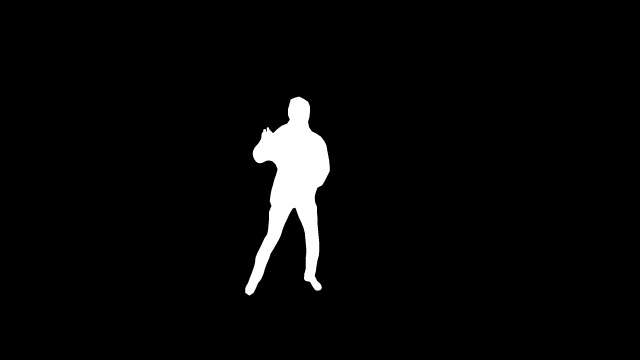} \\ 
   
    \includegraphics[width=0.45\linewidth]{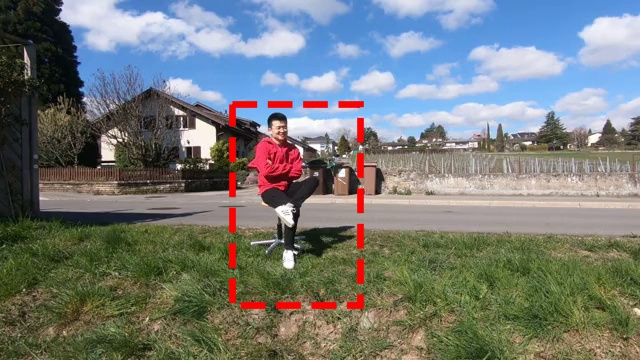}
   \includegraphics[width=0.45\linewidth]{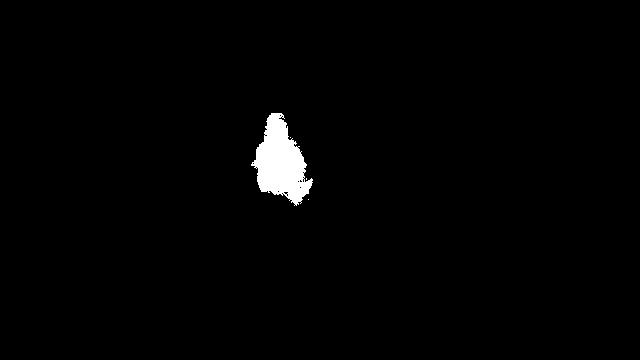}&
   
   \includegraphics[width=0.45\linewidth]{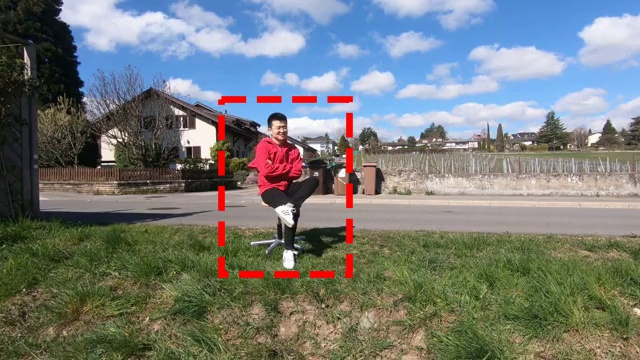} 
   \includegraphics[width=0.45\linewidth]{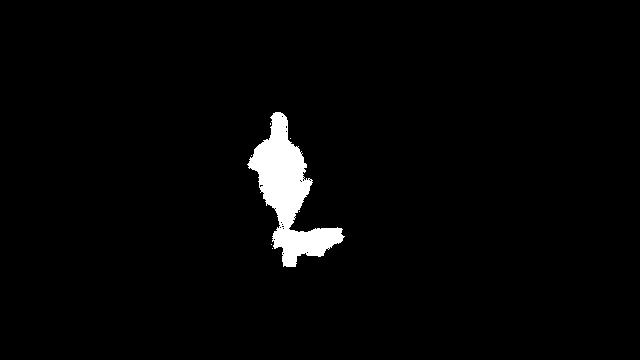} &
   
   \includegraphics[width=0.45\linewidth]{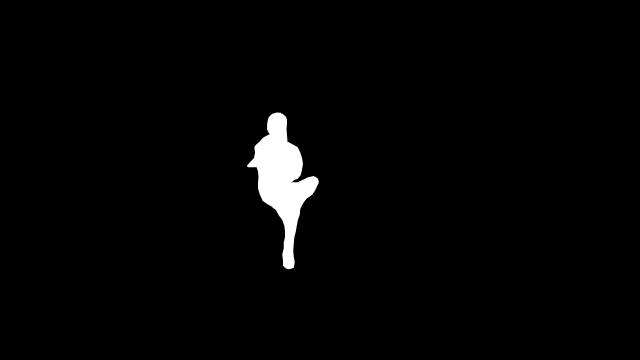} \\ 
   
    \includegraphics[width=0.45\linewidth]{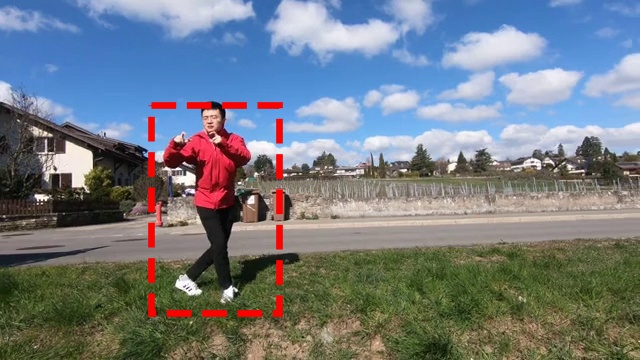}
   \includegraphics[width=0.45\linewidth]{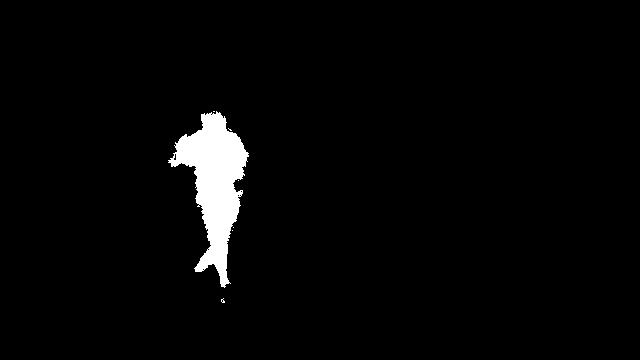}&
   
   \includegraphics[width=0.45\linewidth]{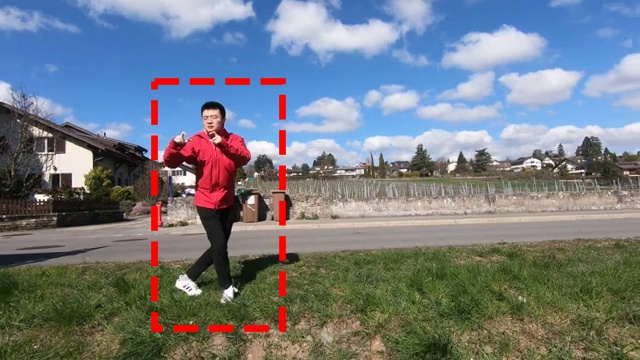} 
   \includegraphics[width=0.45\linewidth]{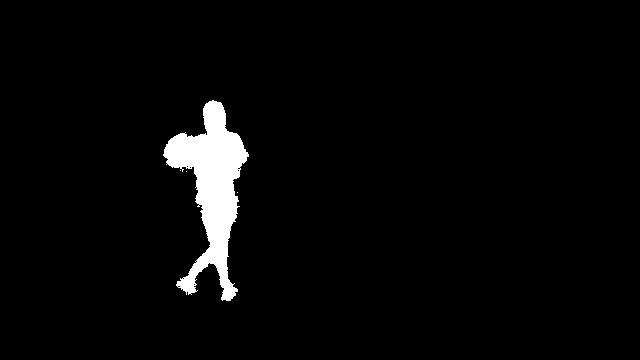} &
   
   \includegraphics[width=0.45\linewidth]{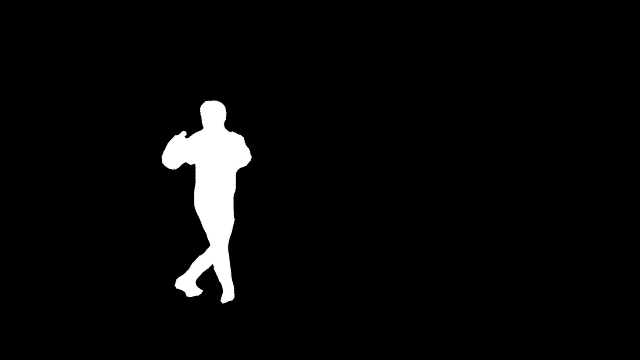} \\ 
   
    \includegraphics[width=0.45\linewidth]{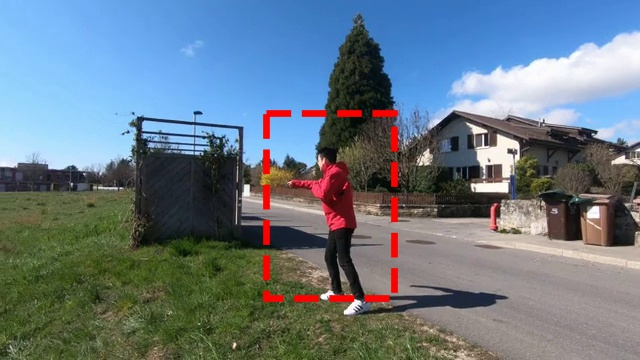}
   \includegraphics[width=0.45\linewidth]{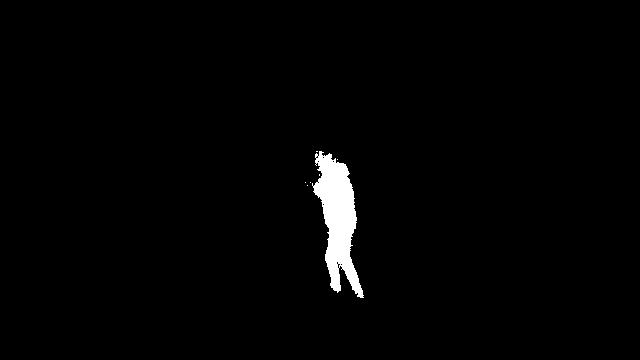}&
   
   \includegraphics[width=0.45\linewidth]{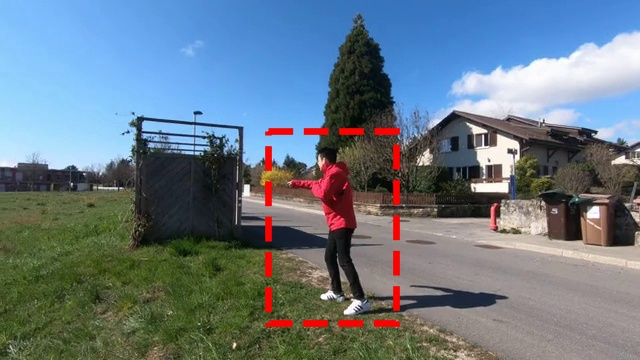} 
   \includegraphics[width=0.45\linewidth]{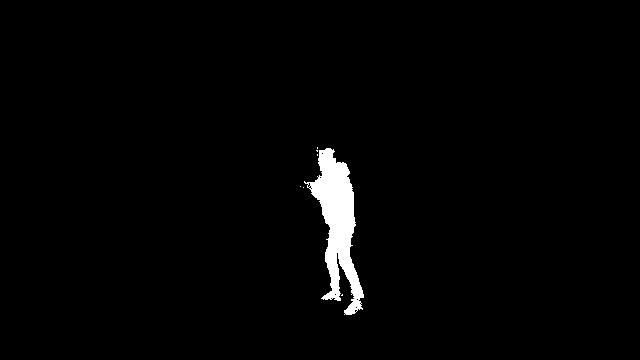} &
   
   \includegraphics[width=0.45\linewidth]{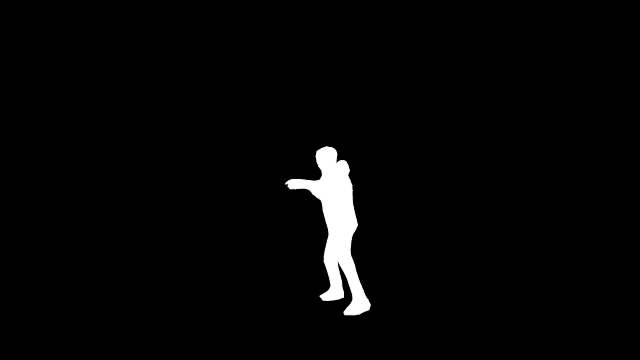} \\

     \includegraphics[width=0.45\linewidth]{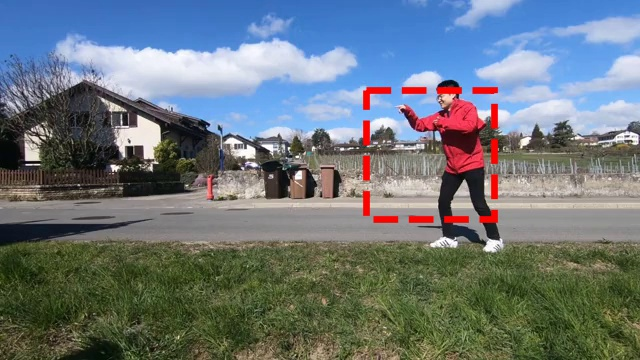}
   \includegraphics[width=0.45\linewidth]{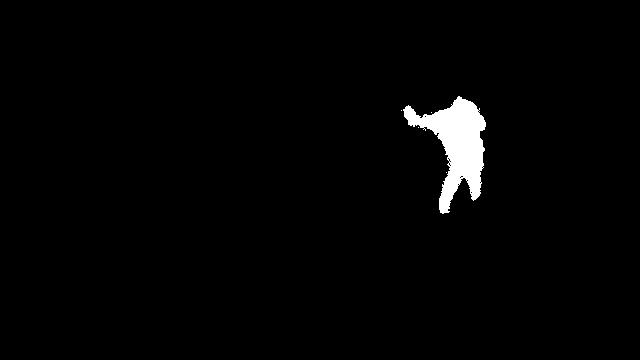}&
   
   \includegraphics[width=0.45\linewidth]{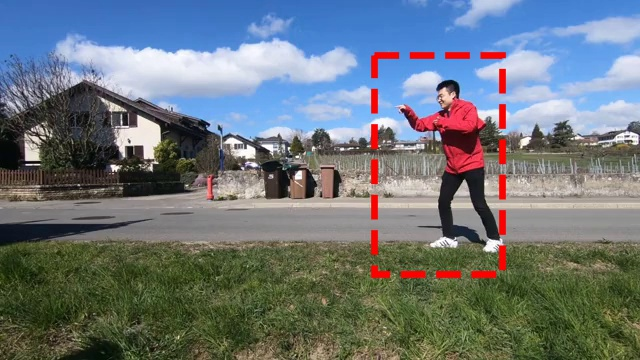} 
   \includegraphics[width=0.45\linewidth]{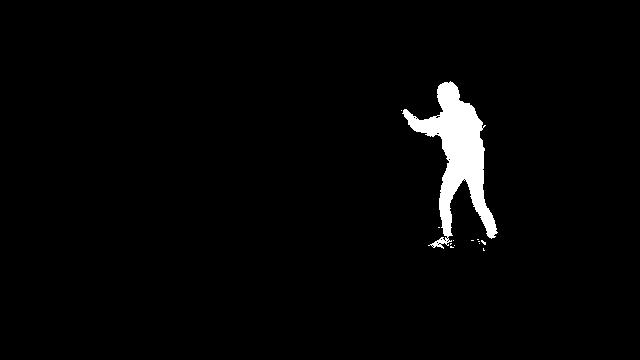} &
   
   \includegraphics[width=0.45\linewidth]{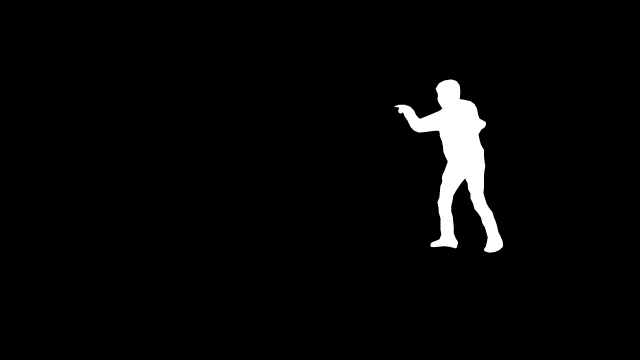} \\

    \includegraphics[width=0.45\linewidth]{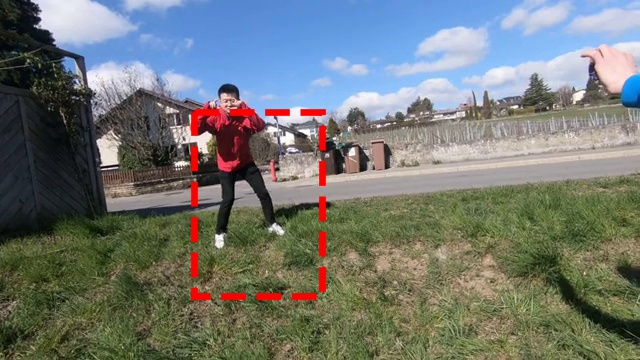}
   \includegraphics[width=0.45\linewidth]{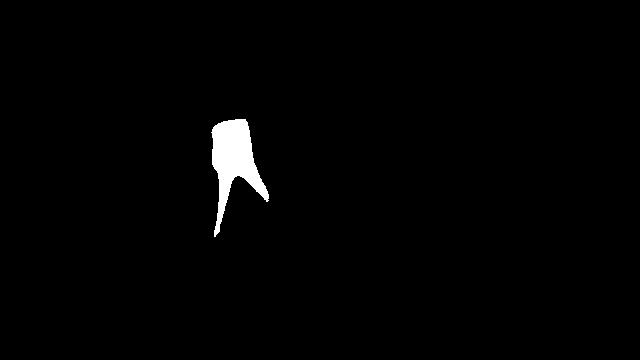}&
   
   \includegraphics[width=0.45\linewidth]{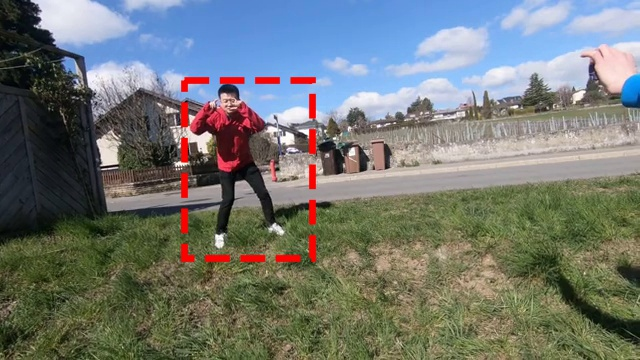} 
   \includegraphics[width=0.45\linewidth]{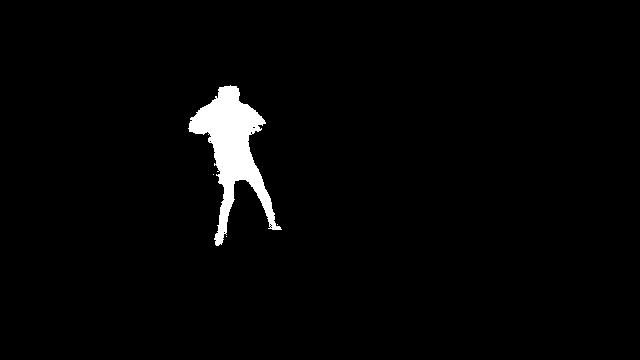} &
   
   \includegraphics[width=0.45\linewidth]{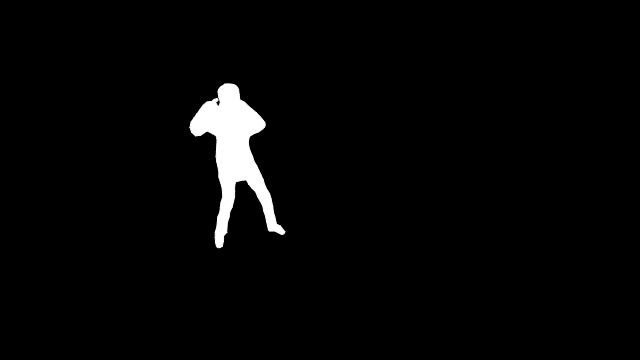} \\

    \includegraphics[width=0.45\linewidth]{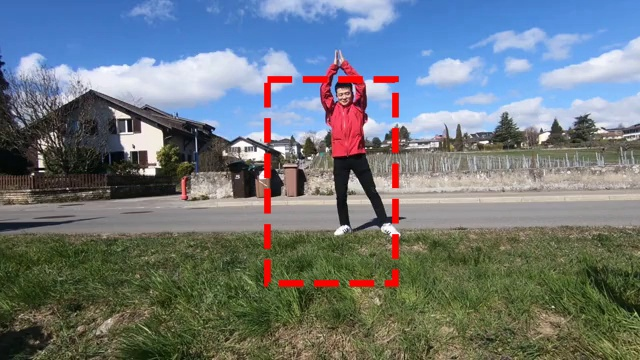}
   \includegraphics[width=0.45\linewidth]{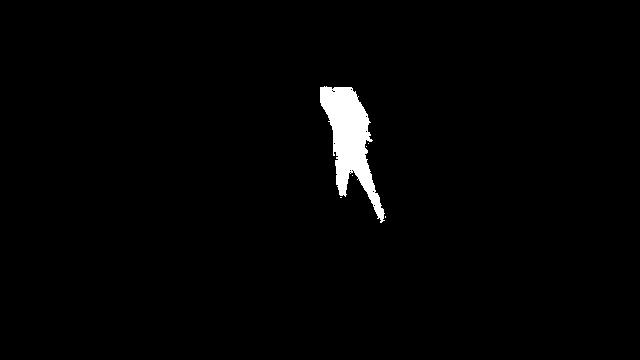}&
   
   \includegraphics[width=0.45\linewidth]{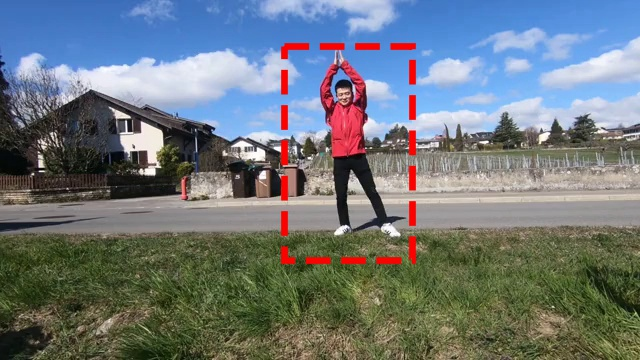} 
   \includegraphics[width=0.45\linewidth]{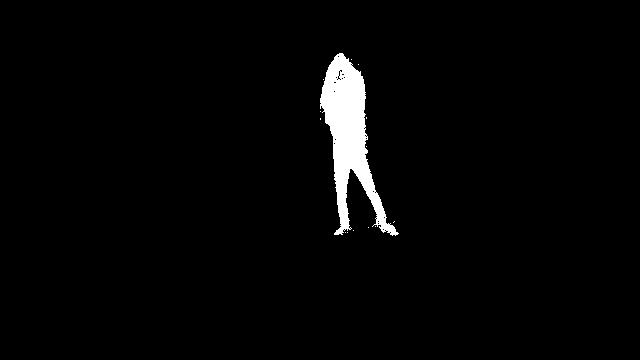} &
   
   \includegraphics[width=0.45\linewidth]{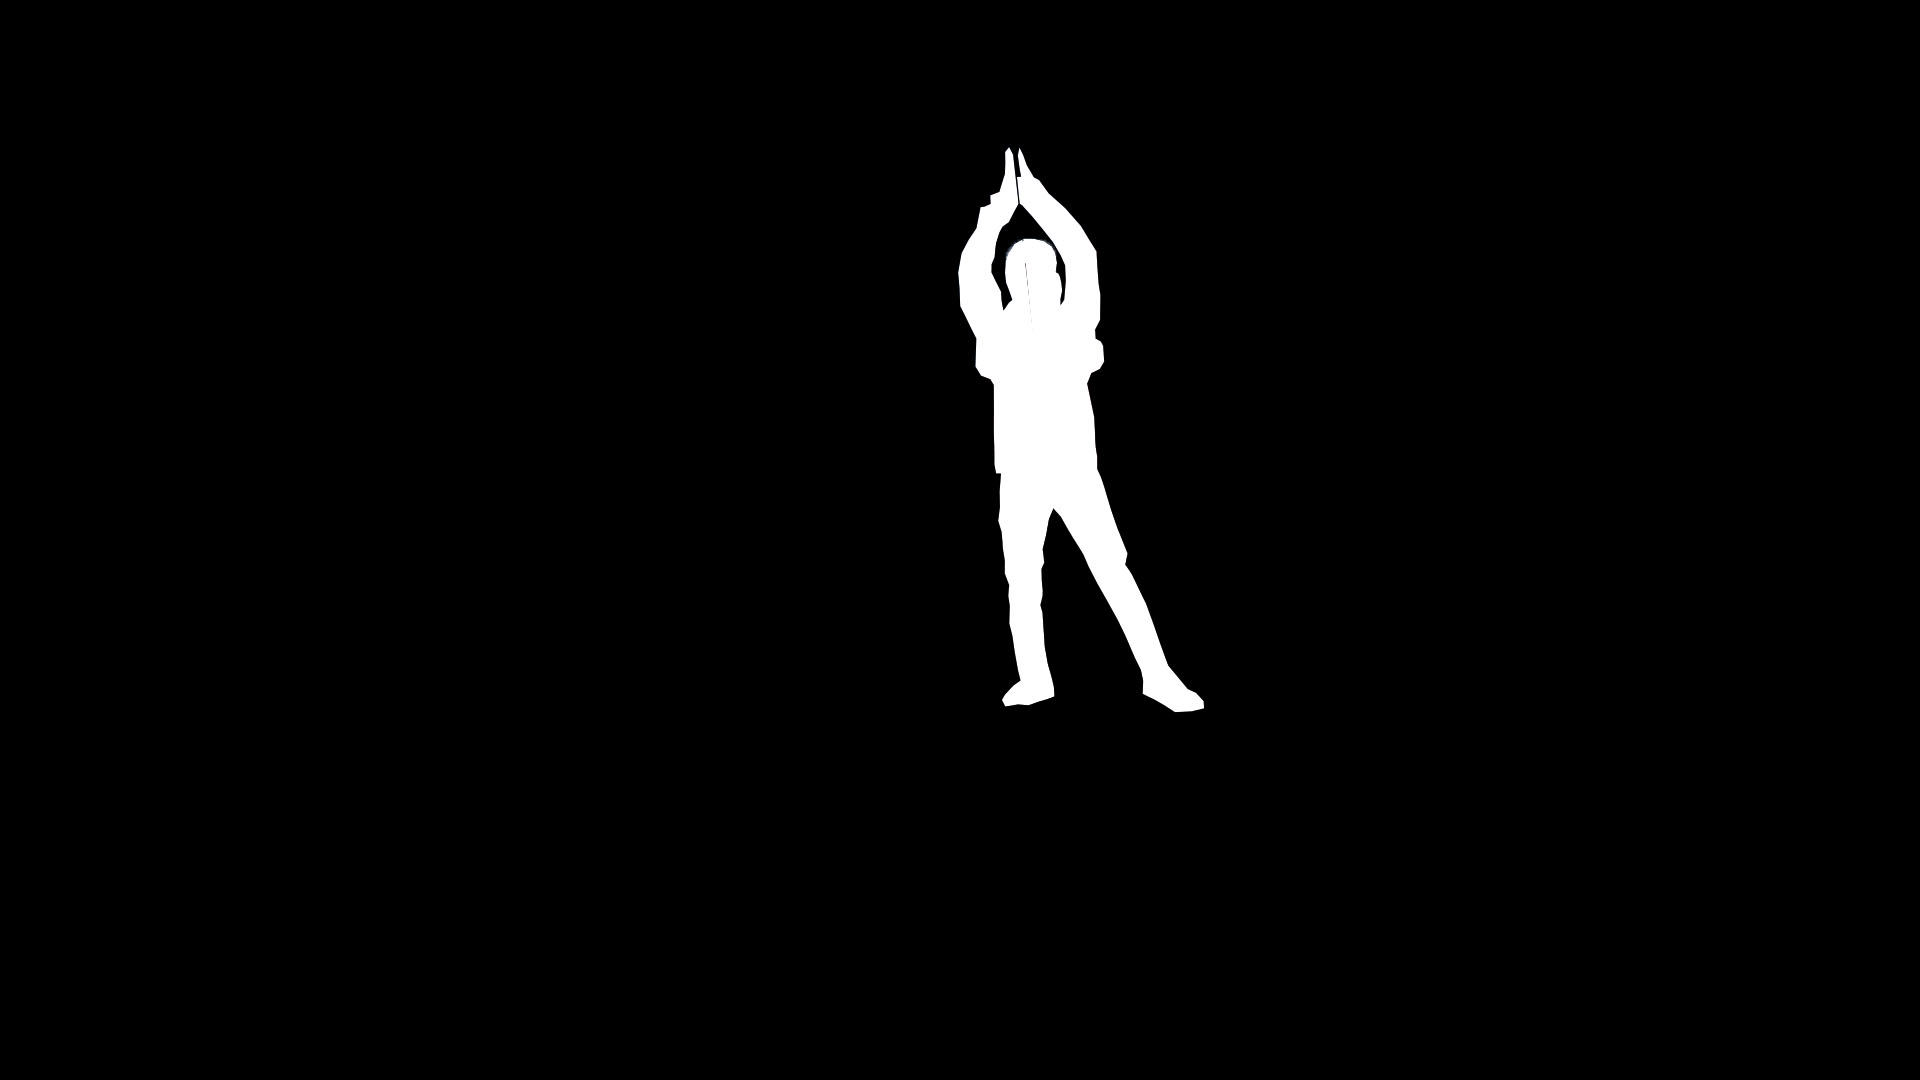} \\ \\ \\

{ \fontsize{22}{5}\selectfont  (a)~Katircioglu et al.~\cite{Katircioglu20}} &  {\fontsize{22}{5}\selectfont  (b) Ours}  & {\fontsize{22}{5}\selectfont  (c) GT }  \\ 
  \end{tabular}}
}

  \caption{\textbf{Qualitative results on the {\handheld{}} dataset.} (a) The detection and segmentation mask results of~\cite{Katircioglu20} trained and tested on single images. (b) The predictions of our model trained using 3-camera multi-view consistency and tested on single images. (c) Ground truth. Our results are generally more accurate, which justifies the effort invested in calibrating the cameras.}
  \label{fig:supp_handheld_qual}
\end{figure*}

\clearpage

\noindent during training, whereas~\cite{Koh17b} uses strong temporal cues both during training and test time and ~\cite{Katircioglu20} leverages optical flow images during training. Due to the background objective, our approach favors tight bounding boxes around the subject and this causes the auxiliary object moving with the primary one to be partially included in the detection. Therefore, compared to the ground truth masks, our predictions do not contain the skis entirely. However, compared to other baselines, our method can segment out the skis more precisely.

On \human{} dataset, our method has more accurate hand detections and lower legs are more precisely segmented compared to~\cite{Katircioglu20} employing a single view approach with optical flow images during training and~\cite{Rhodin19a} using multi-view images during training for novel view synthesis. Even in the rare cases of performing an action on the floor, our method can still reliably detect the person. The failure cases include the detections that miss the head and feet when the chair is in close proximity to the subject. This is expected since the chair is also hard to be reconstructed from its neighboring regions and can be treated as a foreground object.

To demonstrate that our method can be applied to in-the-wild scenes without initial camera calibration, we used the OpenSFM software to calibrate 4200 frames out of 120000 training images in the \handheld{} dataset. We ran OpenSFM with HaHOG (the combination of Hessian Affine feature point detector and HOG descriptor) features and the calibration took approximately 7 hours. We did not provide masks for the moving objects. Nonetheless, we managed to obtain accurate camera poses. Our results in Fig.~\ref{fig:supp_handheld_qual} show that when trained with a small calibrated part of the training set, our multi-view approach can detect and segment the person more accurately than~\cite{Katircioglu20} which often fails to detect the moving object precisely.

Although we target the detection of a single object or person, our probabilistic framework can handle several of them at test time by sampling more than once. In Fig.~\ref{fig:multiperson}, we show an example of this on \ski{}, by synthetically creating an image with two skiers. Our method trained on single person images can accurately detect and segment two skiers as long as they are sufficiently separated.
\begin{figure}[H]
	\centering

	\begin{tabular}{@{}cc@{}}
		
		\includegraphics[width=0.47\linewidth]{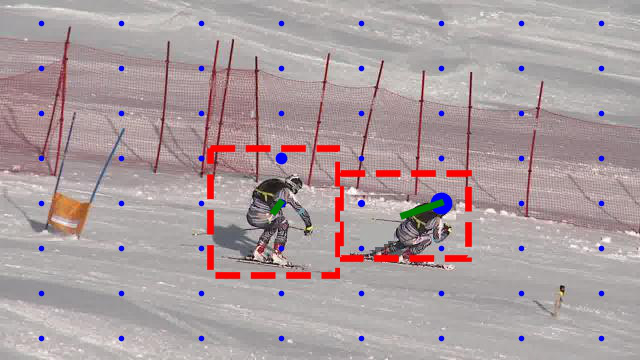} &
		\includegraphics[width=0.47\linewidth]{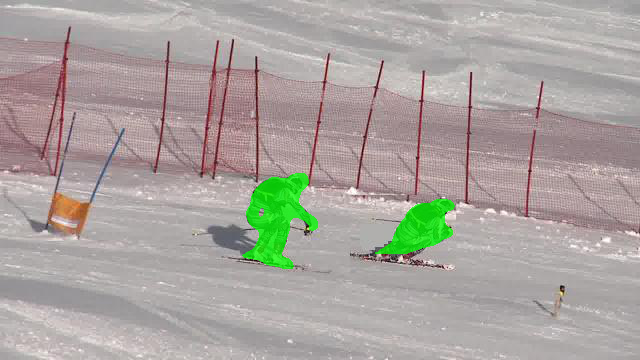}\\
		{\small (a) Detection} &  {\small (b) Segmentation} 
	\end{tabular}
	\caption{Multi-person detection and segmentation at test time.}
	\label{fig:multiperson}

\end{figure}
